# Supplementary material for: DynEval: Holistic Evaluations of T2I Generative Models in the Wild
Source: arXiv:2607.11199 source file (2026-07-13)
Supplement: Supplementary file 1 [file supp.tex]

\newpage
\appendix
\makeatletter

\makeatother

\setcounter{figure}{0}
\setcounter{table}{0}
\setcounter{equation}{0}

\section*{Supplementary Material for DynEval: Holistic Evaluations of T2I Generative
Models in the Wild}
\label{sec:appendix}

\makeatletter
{%
\newcommand{\tocentry}[3]{%
  \par\noindent
  \setlength{\rightskip}{1.5em}%
  \setlength{\parfillskip}{-\rightskip}%
  \textbf{#1}\hspace{6pt}#3%
  \nobreak
  \leaders\hbox{$\m@th\mkern 4.5mu\hbox{.}\mkern 4.5mu$}\hfill
  \nobreak
  \hb@xt@1.5em{\hss\pageref{#2}}\par
  \vspace{2pt}%
}%
\newcommand{\tocsubentry}[3]{%
  \par\noindent
  \setlength{\rightskip}{1.5em}%
  \setlength{\parfillskip}{-\rightskip}%
  \hspace{1.8em}\textbf{#1}\hspace{6pt}#3%
  \nobreak
  \leaders\hbox{$\m@th\mkern 4.5mu\hbox{.}\mkern 4.5mu$}\hfill
  \nobreak
  \hb@xt@1.5em{\hss\pageref{#2}}\par
  \vspace{2pt}%
}%
\vspace{4pt}%
\noindent\textbf{Table of Contents}\\
\vspace{-4pt}
\noindent\rule{\linewidth}{0.5pt}%
\vspace{6pt}%
\tocentry{A}{supp:dataset_Details}{Benchmark Dataset Details}
\tocentry{B}{supp:model_details}{Detailed Information of T2I Models}
\tocentry{C}{supp:cbs}{Complexity Based Scoring}
\tocentry{D}{supp:pt}{Prompt Tiering}
\tocentry{E}{supp:mt}{Model Tiering}
\tocentry{F}{supp:tst}{Details on Tier-Specific Thresholds}
\tocentry{G}{supp:aas}{Additional Ablation Study}
\tocsubentry{G.1}{supp:teacher_choice}{Teacher Model Selection}
\tocsubentry{G.2}{supp:data_scaling}{Training Data Scaling}
\tocentry{H}{supp:added_visual_results}{Additional Qualitative Results}
\tocentry{I}{supp:failure}{Understanding Failure Attributes of T2I Models}
\noindent\rule{\linewidth}{0.5pt}%
\vspace{8pt}%
}
\makeatother

\section{Benchmark Dataset Details}
\label{supp:dataset_Details}

\begin{table*}[t]
\centering
\caption{
\textbf{Statistics of existing T2I evaluation benchmarks.} \grayhl{\textbf{\#Prompts}} denotes the number of unique prompts, \grayhl{\textbf{\#Pairs}} the total number of image-text pairs, \grayhl{\textbf{Images/T2I}} the average number of images contributed by each T2I generative model, and \grayhl{\textbf{\#T2I}} the total number of T2I models evaluated in each benchmark. For \grayhl{\textbf{Prompt Length}}, we report the minimum, maximum, and mean $\pm$ standard deviation ($\mu \pm \sigma$), computed over the number of characters in each prompt, including whitespace and punctuation. \textbf{Mixed} in the \textbf{Images/T2I} column indicates that the number of images contributed by each model varies; therefore, a single images-per-model value cannot be reported. The blank entry for RichHF in the \textbf{Images/T2I} column indicates that RichHF does not provide T2I model metadata for the generated images; therefore, a per-model image count cannot be reported.
}
\label{tab:benchmark_statistics}
\vspace{-3mm}
\small
\setlength{\tabcolsep}{5pt}
\resizebox{\textwidth}{!}{
\begin{tabular}{r|l|l|l|l|l|l|r}
\toprule
\multirow{2}{*}{\textbf{Benchmark}} &
\multirow{2}{*}{\textbf{\#Prompts}} &
\multirow{2}{*}{\textbf{\#Pairs}} &
\multicolumn{3}{c|}{\textbf{Prompt Length}} &
\multirow{2}{*}{\textbf{Images/T2I}} &
\multirow{2}{*}{\textbf{\#T2I}} \\
\cmidrule(lr){4-6}
& & &
\textbf{Min} &
\textbf{Max} &
\textbf{$\mu \pm \sigma$} &
& \\
\midrule
T2I-CoReBench~\cite{T2I-CoReBench}   & 1,080 & 4,320  & 238 & 2,064 & 764.62 $\pm$ 324.51 & 1,080 & 4 \\
TIIF-Bench~\cite{tiff_bench} & 529   & 2,216  & 27  & 2,478 & 358.75 $\pm$ 387.44 & 554   & 4 \\
UniGenBench++~\cite{unigenbench++} & 600   & 3,587  & 64  & 300   & 158.60 $\pm$ 33.81  & Mixed & 6 \\
LMM4LMM~\cite{lmm4lmm_evalmi-50k} & 2,086 & 10,080 & 16  & 1,876 & 98.26 $\pm$ 145.32  & 420   & 24 \\
RichHF~\cite{liang2024rich} & 493   & 955    & 4   & 1,018 & 79.31 $\pm$ 110.69  & --    & 3 \\
EvalMuse~\cite{EvalMuse-40k}        & 989   & 10,796 & 6   & 335   & 68.62 $\pm$ 45.04   & Mixed & 20 \\
GenAI-Bench~\cite{li2024genai}     & 1,600 & 9,600  & 14  & 192   & 67.42 $\pm$ 26.89   & 1,600 & 6 \\
TIFA~\cite{tifa} & 160   & 800    & 13  & 182   & 56.13 $\pm$ 26.90   & 160   & 5 \\
T2I-Eval-Bench~\cite{t2i_eval_bench}  & 8,772 & 8,772  & 25  & 217   & 54.19 $\pm$ 12.54   & Mixed & 3 \\
GenEval 2~\cite{geneval2}        & 800   & 3,200  & 13  & 93    & 50.82 $\pm$ 18.41   & 800   & 4 \\
GenEval~\cite{GenEval} & 100   & 1,200  & 16  & 54    & 31.19 $\pm$ 9.46    & 400   & 3 \\
\bottomrule
\end{tabular}
}
\vspace{-2mm}
\end{table*}

\myparagraph{\textit{Benchmark Dataset Statistics.}} We evaluate \textbf{DynEval} on a diverse collection of 11 text-to-image (T2I) evaluation benchmarks spanning: \textbf{(i)} attribute binding, counting, and spatial relations (GenEval~\cite{GenEval}, GenEval2~\cite{geneval2}, TIFA~\cite{tifa}, and GenAI-Bench~\cite{li2024genai}); \textbf{(ii)} long-form instruction following and complex multi-object interactions (TIIF-Bench~\cite{tiff_bench} and UniGenBench++~\cite{unigenbench++}); \textbf{(iii)} text and symbol rendering (TIIF-Bench~\cite{tiff_bench} and EvalMi~\cite{lmm4lmm_evalmi-50k}); \textbf{(iv)} complex compositional understanding and reasoning (T2I-CoReBench~\cite{T2I-CoReBench}); and \textbf{(v)} human preference evaluations (RichHF~\cite{liang2024rich}). These benchmarks cover a broad spectrum of challenges encountered in modern T2I evaluation, thereby providing complementary testbeds for assessing the robustness and generalization of automatic T2I evaluators. \cref{tab:benchmark_statistics} summarizes the corresponding benchmark statistics, including dataset scale, prompt length, and coverage of T2I models. Specifically, the number of unique prompts ranges from 100 (GenEval~\cite{GenEval}) to 8,772 (T2I-Eval-Bench~\cite{t2i_eval_bench}), while the number of image-text pairs varies from 800 (TIFA~\cite{tifa}) to 10,796 (EvalMuse~\cite{EvalMuse-40k}). Furthermore, prompt complexity varies considerably across benchmarks: the average prompt length ranges from $31.19$ in GenEval~\cite{GenEval} to $764.62$ in T2I-CoReBench~\cite{T2I-CoReBench}, reflecting the recent trend toward increasingly long and semantically complex prompts. In our analysis, prompt length is measured as the number of characters in each prompt, including whitespace and punctuation. Likewise, the number of generated images per T2I model and the number of evaluated models vary substantially across benchmarks, with the latter ranging from 3 to 24 models. Collectively, these statistics demonstrate that our evaluation encompasses a diverse range of benchmark characteristics, enabling a comprehensive assessment of \textbf{DynEval}'s robustness and generalization across varying prompt complexities and image generation scenarios.

\myparagraph{\textit{Human Annotations.}} As noted in the main paper, GenEval2~\cite{geneval2}, TIIF-Bench~\cite{tiff_bench}, UniGenBench++~\cite{unigenbench++}, and T2I-CoReBench~\cite{T2I-CoReBench} do not provide publicly available human annotations. Moreover, GenEval2~\cite{geneval2} does not release the images used in its evaluation protocol. To facilitate evaluation on GenEval2, we generate images for its 800 evaluation prompts using four recent text-to-image generative models, namely GPT-Image-1.5~\cite{gpt_image_1_5}, NanoBanana~\cite{team2023gemini}, Qwen-Image~\cite{wu2025qwen}, and FLUX.2 [dev]~\cite{flux-2-2025}, resulting in 3,200 prompt-image pairs. We then collect human annotations for all four benchmarks using a unified annotation protocol. Since our objective is to evaluate both text-to-image alignment (T2IA) and image quality assessment (IQA), we adopt an attribute-centric annotation strategy inspired by EvalMuse~\cite{EvalMuse-40k}. Specifically, for each prompt-image pair, we decompose the input prompt into a set of atomic semantic attributes. Annotators are then presented with the prompt, the generated image, and the complete set of semantic attributes specified in the prompt, including objects, attributes, actions, counts, and spatial relations. For each semantic attribute, annotators assign a binary label: a score of 0 indicates that the generated image fails to satisfy the corresponding attribute, whereas a score of 1 indicates that the image successfully satisfies the attribute. This fine-grained annotation protocol enables a comprehensive assessment of semantic faithfulness while providing a principled proxy for perceptual image quality through aggregated attribute-level annotations. Finally, we compute a human score for each prompt-image pair by averaging the binary attribute labels, yielding a normalized score in the range $[0,1]$. Although multiple annotators per sample are generally preferred for improving annotation reliability, we employ a single annotator per sample due to practical resource constraints. We emphasize that the primary purpose of these annotations is not to introduce new human-annotated benchmarks, but rather to enable a rigorous evaluation of the proposed \textbf{DynEval} on recent and increasingly challenging T2I evaluation benchmarks.

\section{Detailed Information of T2I Models}
\label{supp:model_details}

\begin{table*}[!ht]
\centering
\scriptsize
\caption{\textbf{Overview of the 36 T2I generative models used in DynEval.} The selected models span five years of progress in image generation (2022--2026), covering early diffusion models, diffusion transformers (DiTs), autoregressive image generation models, unified multimodal generative models, and recent large-scale foundation models. For each model, we report its release date (Year.Month), native image generation resolution, and the URL of its official repository or model release.}
\label{tab:t2i_models}
\vspace{-2mm}
\setlength{\tabcolsep}{3pt}

\begin{tabularx}{\textwidth}{l c r X}
\toprule
\textbf{Model} & \textbf{Release} & \textbf{Resolution} & \textbf{URL} \\
\midrule

Stable Diffusion v1.5 & 2022.01 & $512\times512$ & \url{https://huggingface.co/stable-diffusion-v1-5/stable-diffusion-v1-5} \\
Kandinsky 3           & 2022.11 & $1024\times1024$ & \url{https://github.com/ai-forever/kandinsky-3} \\
Stable Diffusion v2.1 & 2022.12 & $768\times768$   & \url{https://huggingface.co/sd2-community/stable-diffusion-2-1} \\
\midrule

SSD-1B                & 2023.01 & $1024\times1024$ & \url{https://huggingface.co/segmind/SSD-1B} \\
DeepFloyd IF-XL       & 2023.04 & $64\times64$     & \url{https://huggingface.co/DeepFloyd/IF-I-XL-v1.0} \\
Stable Diffusion XL   & 2023.07 & $1024\times1024$ & \url{https://huggingface.co/stabilityai/stable-diffusion-xl-base-1.0} \\
PixArt-$\alpha$          & 2023.09 & $1024\times1024$ & \url{https://github.com/PixArt-alpha/PixArt-alpha} \\
SDXL-Turbo            & 2023.11 & $512\times512$   & \url{https://huggingface.co/stabilityai/sdxl-turbo} \\
\midrule

Playground v2.5       & 2024.02 & $1024\times1024$ & \url{https://huggingface.co/playgroundai/playground-v2.5-1024px-aesthetic} \\
PixArt-$\Sigma$          & 2024.04 & $1024\times1024$ & \url{https://huggingface.co/PixArt-alpha/PixArt-Sigma-XL-2-1024-MS} \\
Hunyuan-DiT           & 2024.06 & $1024\times1024$ & \url{https://github.com/Tencent-Hunyuan/HunyuanDiT} \\
LlamaGen              & 2024.06 & $256\times256$   & \url{https://github.com/foundationvision/llamagen} \\
Kolors                & 2024.07 & $1024\times1024$ & \url{https://github.com/Kwai-Kolors/Kolors} \\
FLUX.1 [dev]            & 2024.08 & $1024\times1024$ & \url{https://huggingface.co/black-forest-labs/FLUX.1-dev} \\
Show-o                & 2024.08 & $256\times256$   & \url{https://github.com/showlab/show-o} \\
OmniGen               & 2024.09 & $1024\times1024$ & \url{https://github.com/vectorspacelab/omnigen} \\
Emu3                  & 2024.09 & $720\times720$   & \url{https://github.com/baaivision/emu3} \\
Stable Diffusion 3.5  & 2024.10 & $1024\times1024$ & \url{https://huggingface.co/stabilityai/stable-diffusion-3.5-large} \\
Sana                  & 2024.11 & $1024\times1024$ & \url{https://huggingface.co/Efficient-Large-Model/Sana_1600M_1024px} \\
In-Context LoRA       & 2024.12 & $1024\times1024$ & \url{https://huggingface.co/ali-vilab/In-Context-LoRA} \\
\midrule

Janus-Pro             & 2025.01 & $384\times384$   & \url{https://huggingface.co/deepseek-ai/Janus-Pro-7B} \\
HiDream-I1            & 2025.04 & $1024\times1024$ & \url{https://huggingface.co/HiDream-ai/HiDream-I1-Full} \\
Bagel                 & 2025.05 & $1024\times1024$ & \url{https://github.com/bytedance-seed/BAGEL} \\
OmniGen2              & 2025.06 & $1024\times1024$ & \url{https://github.com/VectorSpaceLab/OmniGen2} \\
UniWorld-V1           & 2025.06 & $1024\times1024$ & \url{https://github.com/PKU-YuanGroup/UniWorld/tree/main/UniWorld-V1} \\
UniPic                & 2025.07 & $1024\times1024$ & \url{https://github.com/SkyworkAI/UniPic/tree/main/UniPic-1} \\
Qwen-Image            & 2025.08 & $1328\times1328$ & \url{https://huggingface.co/Qwen/Qwen-Image} \\
X-Omni                & 2025.08 & $1024\times1024$ & \url{https://github.com/X-Omni-Team/X-Omni} \\
FLUX.2 [dev]            & 2025.11 & $1024\times1024$ & \url{https://huggingface.co/black-forest-labs/FLUX.2-dev} \\
FIBO                  & 2025.11 & $1024\times1024$ & \url{https://huggingface.co/briaai/FIBO} \\
GPT-Image-1.5         & 2025.12 & $1024\times1024$ & \url{https://developers.openai.com/api/docs/models/gpt-image-1.5} \\
LongCat-Image         & 2025.12 & $1024\times1024$ & \url{https://huggingface.co/meituan-longcat/LongCat-Image} \\
\midrule

FLUX.2 [klein]          & 2026.01 & $1024\times1024$ & \url{https://huggingface.co/black-forest-labs/FLUX.2-klein-9B} \\
GLM-Image             & 2026.01 & $1024\times1024$ & \url{https://huggingface.co/zai-org/GLM-Image} \\
Z-Image               & 2026.01 & $1024\times1024$ & \url{https://huggingface.co/Tongyi-MAI/Z-Image} \\
NanoBanana            & 2026.02 & $1024\times1024$ & \url{https://nanobanana.gg/} \\

\bottomrule
\end{tabularx}
\end{table*}

To construct \textbf{GenDB} and \textbf{DynEvalInstruct}, we consider a diverse collection of \textbf{36} text-to-image (T2I) generation models spanning five years of progress (2022 to 2026) in image generation. Our model pool covers: \textbf{(i)} \textbf{early diffusion-based models} such as Stable Diffusion~v1.5~\cite{rombach2022high}, Stable Diffusion~v2.1~\cite{rombach2022high}, Kandinsky~3~\cite{arkhipkin2023kandinsky}, and DeepFloyd IF-XL~\cite{deepfloydif2023}; \textbf{(ii) diffusion transformer (DiT)} models such as PixArt-$\alpha$~\cite{chen2023pixart}, Hunyuan-DiT~\cite{li2024hunyuan_dit}, FLUX.1 [dev]~\cite{flux2024}, FLUX.2 [dev]~\cite{flux-2-2025}, LongCat-Image~\cite{LongCat-Image}, GLM-Image~\cite{glmimage2024}, and Z-Image~\cite{team2025zimage}; \textbf{(iii) autoregressive image generation} models, including LlamaGen~\cite{sun2024autoregressive} and Show-o~\cite{xie2024show}; \textbf{(iv) unified multimodal generative models} such as OmniGen~\cite{xiao2025omnigen}, OmniGen2~\cite{wu2025omnigen2}, Emu3~\cite{wang2024emu3}, Janus-Pro~\cite{chen2025janus}, UniWorld-V1~\cite{lin2025uniworld}, UniPic~\cite{wang2025skywork}, and X-Omni~\cite{geng2025x}; \textbf{(v) recent open-source foundation models} such as Qwen-Image~\cite{wu2025qwen}; and \textbf{(vi) closed-source models} including \texttt{GPT-Image-1.5}~\cite{gpt_image_1_5} and \texttt{NanoBanana}~\cite{team2023gemini}. The complete list of models, along with their release dates, native generation resolutions, and official URLs, is provided in Tab.~\ref{tab:t2i_models}.

To estimate the generation capability of these models, we construct the \textbf{DynEval-1K} evaluation set, comprising 1,000 prompts sampled to cover 42 prompt subcategories across 9 semantic dimensions. Each T2I model generates one image per prompt, yielding 1,000 prompt-image pairs per model. We report the average DynEval-4B predicted score across these 1,000 prompt-image pairs as the overall capability score of each model in Tab.~\ref{tab:dyneval_models}.

\begin{table}[!t]
\centering
\caption{\textbf{Example prompts from the three prompt-complexity tiers in GenDB}. The prompts are sampled from 500K human-written prompts collected from DiffusionDB~\cite{DiffusionDB}, a large-scale dataset containing approximately 1.8M prompts, and are categorized by complexity. \grayhl{\textbf{Tier-1}} contains long, compositionally rich prompts that require complex semantic reasoning; \grayhl{\textbf{Tier-2}} contains prompts of moderate complexity; and \grayhl{\textbf{Tier-3}} consists of short, relatively simple prompts. These tiers are used in the tier-matched prompt-model generation strategy described in \cref{sec:gendb} of the main paper.
}

\footnotesize
\setlength{\tabcolsep}{5pt}

\begin{tabularx}{\linewidth}{p{2cm} X}
\toprule
\textbf{Tier} & \textbf{Prompt} \\
\midrule

&
\textbf{\underline{Prompt-1:}} A dramatic beautiful sketch concept painting of short curly hair male profile wearing astronaut helmet and headphones in the style of norman rockwell, 1920's, curious or suspicious expression, digital painting, concept art, fine art, cinematic lighting, red, white and blue color scheme, vivid colors, art by norman rockwell \\

Tier-1 &
\textbf{\underline{Prompt-2:}} A beautiful girl sitting in her office petting a cat in her lap, cute -- fine -- subtle smile, face, red hair, pretty face, fine details by stanley artgerm lau, wlop, rossdraws, james jean, andrei riabovitchev, marc simonetti, and sakimichan, trending on artstation \\

&
\textbf{\underline{Prompt-3:}} A cinematic joyous closeup moment of two school friends enjoying life in a ski cafe and visiting wearing boho clothing peonies, boy girl traditional romance, full body portrait, artwork by doja cat, charlie bowater, waterhouse, greg rutkowski, wong kar wai, bestselling movie poster, official media, pixiv, 1990s fashion, official anime media, artstation concept \\

\midrule

&
\textbf{\underline{Prompt-1:}} Concept art for a video game, inside of a futuristic but classy mansion, style of Blade Runner and Mirror's Edge, anime, isometric perspective \\

Tier-2 &
\textbf{\underline{Prompt-2:}} Illustration of a hand controlling puppet strings behind red theater curtains, marionette silhouette visible, dramatic stage composition, deep shadows, very dark moody ambiance, cinematic lighting, highly detailed, textured illustration, album cover art style \\

&
\textbf{\underline{Prompt-3:}} A teddy bear wearing business casual clothes sitting on a couch, 4K photo \\

\midrule

&
\textbf{\underline{Prompt-1:}} Oil painting of someone sitting in a big room, sad, surrounded by books \\

Tier-3 &
\textbf{\underline{Prompt-2:}} A painting of a couple looking at each other in low light, it is so dark you can barely make out their features \\

&
\textbf{\underline{Prompt-3:}} A puffin sitting in booth while eating a pastry at a diner, etching \\

\bottomrule
\end{tabularx}
\label{tab:tier_prompts}
\end{table}

\section{Complexity Based Scoring}
\label{supp:cbs}

As described in \cref{sec:gendb} of the main paper, we sample prompts of varying complexity from the 1.8M human-written prompts available in DiffusionDB~\cite{DiffusionDB} using a \textit{heuristic scoring strategy} designed to estimate the semantic richness and compositional difficulty of a prompt. This scoring mechanism prioritizes prompts that are more likely to challenge the target T2I models. We first remove all prompts that contain fewer than 30 characters, where the character count includes alphabetic characters, numbers, spaces, and punctuation symbols. This filtering step eliminates overly short prompts that typically lack sufficient semantic content. For each remaining prompt $p$, we compute a score based on \textbf{9} factors capturing different aspects of prompt complexity: \textbf{(i)} prompt length, \textbf{(ii)} object and attribute counts, \textbf{(iii)} compositional density measured by the number of comma-separated clauses, \textbf{(iv)} artist or style attribution patterns (\emph{e.g.}, \textit{`in the style of'}, \textit{`art by'}, \textit{`inspired by'}), \textbf{(v)} technical rendering and fidelity terminology (\emph{e.g.}, rendering engines, lighting conditions, optics, and resolution cues), \textbf{(vi)} explicit detail descriptors (\emph{e.g.}, \textit{`highly detailed'}, \textit{`intricate'}, \textit{`sharp focus'}), \textbf{(vii)} high-level style keywords (\emph{e.g.}, \textit{`cyberpunk'}, \textit{`baroque'}), \textbf{(viii)} color specifications, and \textbf{(ix)} interaction or relational expressions. While prompt length is computed directly, the remaining eight semantic factors are extracted using \texttt{Qwen3-8B} as a metadata extraction model to identify the presence and count of the corresponding attributes in a given prompt. This hybrid design enables efficient extraction of higher-level semantic information while preserving the exact prompt length. After extracting the aforementioned metadata, we compute a \textit{heuristic complexity score} using a weighted linear combination of the nine factors:

\vspace{-2mm}
\begin{equation}
H(p) = \sum_{j=1}^{9} w_j f_j(p),
\vspace{-1mm}
\end{equation}
where $f_j(p)$ denotes the value of the $j$-th complexity attribute associated with prompt $p$. Specifically, $f_1(p)$ is computed directly from prompt length, whereas $f_j(p)$ for $j \in \{2,\ldots,9\}$ are derived from the metadata extracted using \texttt{Qwen3-8B}. The term $w_j$ denotes the weighting coefficient associated with the $j$-th attribute. Based on empirical observations, we found that prompt length ($f_1(p)$) and the number of objects and attributes ($f_2(p)$) are the most reliable indicators of semantic and compositional complexity. Accordingly, we assign higher importance to these two factors by setting their weights (\emph{i.e.}, $w_1$ and $w_2$) to $0.2$, while assigning a weight of $0.1$ to the remaining seven semantic factors:

\vspace{-2mm}
\begin{equation}
w_j =
\begin{cases}
0.2, & j \in \{1,2\},\\
0.1, & j \in \{3,\ldots,9\}.
\end{cases}
\vspace{-0.8mm}
\end{equation}

We note that the absolute values of these weights are not critical, as the scores are used only to derive a relative ranking of prompts (based on $H(\cdot)$). Instead, the key design choice is the relative weighting scheme, which assigns approximately twice the importance to prompt length and object/attribute counts compared to the remaining factors. The resulting score serves as a heuristic estimate of prompt richness and compositional complexity. We compute this score for all \textit{candidate prompts}, rank them accordingly, and subsequently perform the prompt tiering procedure as described in \cref{supp:pt}.
\section{Prompt Tiering}
\label{supp:pt}

Given a set of $N$ candidate prompts $\{p_i\}_{i=1}^{N}$, we first compute a heuristic complexity score $h_i = H(p_i)$ for each prompt, where $H(\cdot)$ denotes the \textit{heuristic complexity scoring function} described in Sec.~\ref{supp:cbs}. We then sort the candidate prompts according to their complexity scores $\{h_i\}_{i=1}^{N}$ and partition the ranked distribution into three tiers corresponding to easy, medium, and hard prompts. This stratification enables \textbf{GenDB} to systematically capture a broad spectrum of semantic and compositional difficulties encountered in real-world text-to-image (T2I) generation. The score boundaries separating these tiers define two adaptive thresholds, $\tau_1$ and $\tau_2$, which are determined empirically from the score distribution rather than specified a priori. Importantly, the choice of $\tau_1$ and $\tau_2$ depends on several factors, including the \textit{size of the candidate prompt pool}, the \textit{desired number of complexity tiers}, and the \textit{capabilities of the target T2I models}. For instance, prompts with high semantic and compositional complexity can disproportionately challenge smaller open-source T2I models, often resulting in severe generation failures. Such prompt-image pairs are generally unsuitable for training the evaluator, as they provide limited opportunity to learn subtle semantic, compositional, and perceptual discrepancies.

Notably, during the construction of \textbf{GenDB}, we analyzed the complexity score distribution of the 1.8M prompts from DiffusionDB~\cite{DiffusionDB} and empirically selected $\tau_1 = 200$ and $\tau_2 = 100$, resulting in three prompt complexity tiers:
\vspace{-2mm}
\begin{equation}
\text{Tier}(p) =
\begin{cases}
\text{Tier-1 (Hard)} & \text{if } H(p) \ge \tau_1, \\
\text{Tier-2 (Medium)} & \text{if } \tau_2 \le H(p) < \tau_1, \\
\text{Tier-3 (Easy)} & \text{otherwise}
\end{cases}
\vspace{-2mm}
\end{equation}

In addition to the complexity-related metadata extraction described in Sec.~\ref{supp:cbs}, we employ \texttt{Qwen3-8B} to annotate each prompt with semantic dimension and subcategory labels based on a predefined taxonomy comprising 9 dimensions and 42 subcategories. Since a real-world prompt can simultaneously encompass multiple semantic concepts (\emph{e.g.}, objects, attributes, actions, spatial relationships, and artistic styles), we adopt a multi-label categorization strategy, assigning all applicable semantic dimensions and subcategory labels to each prompt. These semantic annotations are not used to determine the complexity tiers; rather, they are utilized during prompt selection within each tier. Specifically, after partitioning the 1.8M prompts into three complexity tiers, we perform diversity-aware sampling from each tier while ensuring broad coverage across all 42 semantic subcategories, yielding 500K prompts for \textbf{GenDB}. This strategy prevents the over-representation of frequent prompt types and enables GenDB to capture variations in both semantic content and compositional complexity.

\myparagraph{\textit{Illustrations of Prompt Tiering and Categorization.}}
Tab.~\ref{tab:tier_prompts} presents representative examples from each prompt complexity tier. As expected, Tier-1 primarily contains longer prompts with richer compositional structure and multiple semantic constraints, whereas Tier-3 consists of shorter prompts with relatively simple semantics. Tier-2 lies between these two extremes, containing prompts of moderate length and complexity. Representative examples covering the 42 prompt subcategories grouped under the 9 major semantic dimensions are presented in Tab.~\ref{tab:prompt_cat_1}--Tab.~\ref{tab:prompt_cat_5}. Specifically, Tab.~\ref{tab:prompt_cat_1} presents subcategories belonging to \textit{Object and Entity}; Tab.~\ref{tab:prompt_cat_2} covers \textit{Attribute Binding}; Tab.~\ref{tab:prompt_cat_3} includes \textit{Counting}, \textit{Spatial}, and \textit{Relations}; Tab.~\ref{tab:prompt_cat_4} illustrates \textit{Actions}, \textit{Scene Understanding}, and \textit{Text and Symbols}; and Tab.~\ref{tab:prompt_cat_5} presents subcategories from \textit{Style and Aesthetics}. For each subcategory, a representative prompt is provided, with the corresponding words or phrases highlighted for clarity.
\begin{table}[!t]
\centering
\caption{Illustrative prompts from the \grayhl{\textbf{\textit{Object and Entity}}} semantic dimension, one of the 9 dimensions in the considered prompt taxonomy. Representative prompts from the remaining semantic dimensions are presented in Tab.~\ref{tab:prompt_cat_2}--Tab.~\ref{tab:prompt_cat_5}. Words or phrases corresponding to each subcategory within this dimension are highlighted for clarity.}
\footnotesize
\begin{tabularx}{\textwidth}{p{3.6cm} p{3.6cm} >{\raggedright\arraybackslash}X}
\toprule
\textbf{Prompt Category} & \textbf{Subcategory} & \textbf{Prompt Example} \\
\midrule

Object and Entity & Single Object &
A \hlkw{single wooden chair} placed in the center of a white studio background \\

Object and Entity & Two Objects &
\hlkw{Two vipers entwined}, fighting to the death realistic cinematic 3 5 mm \\

Object and Entity & Human Present &
A portrait of \hlkw{a young woman} reading a book while sitting in a cozy café, warm lighting, coffee cup on the table, realistic photography, shallow depth of field, 8k \\

Object and Entity & Animal Present &
A \hlkw{golden retriever} running through a grassy park under a bright blue sky, joyful expression, motion blur, natural outdoor lighting, highly detailed, 8k photography \\

Object and Entity & Vehicle Present &
A \hlkw{blue sports car} parked beside a mountain road at sunset, cinematic lighting, dramatic clouds, photorealistic render, ultra detailed, 8k \\

Object and Entity & Food Present &
A \hlkw{bowl of ramen} with noodles, eggs, and vegetables on a wooden table, steam rising, food photography, studio lighting, hyper realistic, detailed textures \\

Object and Entity & Plant Present &
A \hlkw{green cactus} growing in a clay pot near a sunny window, minimal interior background, soft natural lighting, ultra detailed botanical photography \\

Object and Entity & Landmark Present &
\hlkw{The Eiffel Tower} illuminated at night with glowing city lights and reflections on the river Seine, cinematic view, long exposure photography, ultra detailed \\

\bottomrule
\end{tabularx}
\label{tab:prompt_cat_1}
\end{table}

\begin{table}[!t]
\centering
\caption{Illustrative prompts from the \grayhl{\textbf{\textit{Attribute Binding}}} semantic dimension, continuing Tab.~\ref{tab:prompt_cat_1}. Words or phrases corresponding to each subcategory within this dimension are highlighted for clarity.}
\footnotesize
\begin{tabularx}{\textwidth}{p{3.6cm} p{3.6cm} >{\raggedright\arraybackslash}X}
\toprule
\textbf{Prompt Category} & \textbf{Subcategory} & \textbf{Prompt Example} \\
\midrule

Attribute Binding & Atomic Color Binding &
A \hlkw{blue bicycle with bright red wheels} parked beside a white wall in a quiet street, vibrant colors, soft shadows, photorealistic, 8k \\

Attribute Binding & Shape Binding &
A \hlkw{triangular yellow kite} with blue stripes flying high in a clear sky above a grassy field, bright daylight, dynamic perspective \\

Attribute Binding & Material Binding &
A \hlkw{glass teapot with a polished metal handle} placed on a marble countertop with soft reflections, studio lighting, macro photography, ultra detailed \\

Attribute Binding & Texture Binding &
A \hlkw{fluffy white pillow} resting on a rough wooden bench inside a rustic cabin, soft sunlight through window, detailed texture contrast \\

Attribute Binding & Size Binding &
A \hlkw{tiny toy robot} standing next to a \hlkw{large cardboard box} on a clean floor, size contrast emphasis, studio lighting, photorealistic \\

Attribute Binding & Style Binding &
A portrait of a woman painted in \hlkw{impressionist style} with vibrant brushstrokes and colorful lighting, inspired by classic impressionist art \\

Attribute Binding & Multi Attribute Binding &
A \hlkw{small green frog wearing a red hat and holding a yellow umbrella} while sitting on a lily pad in a pond, whimsical fantasy illustration \\

\bottomrule
\end{tabularx}
\label{tab:prompt_cat_2}
\end{table}

\begin{table}[!t]
\centering
\caption{Illustrative prompts from the \grayhl{\textbf{\textit{Counting}}}, \grayhl{\textbf{\textit{Spatial}}}, and \grayhl{\textbf{\textit{Relations}}} semantic dimensions, continuing Tab.~\ref{tab:prompt_cat_2}. Words or phrases corresponding to each subcategory within these dimensions are highlighted for clarity.}
\footnotesize
\begin{tabularx}{\textwidth}{p{3.6cm} p{3.6cm} >{\raggedright\arraybackslash}X}
\toprule
\textbf{Prompt Category} & \textbf{Subcategory} & \textbf{Prompt Example} \\
\midrule

Counting & Count Exact &
\hlkw{Five bright oranges} arranged in a straight line on a kitchen table with soft window lighting, photorealistic food photography \\

Counting & Count Approx. &
\hlkw{About twenty birds} flying together across a glowing sunset sky above the ocean, dramatic clouds, cinematic atmosphere \\

Counting & Count Multi Objects &
\hlkw{Three dogs and two cats} sitting together in a cozy living room with a couch and warm lighting, cute and friendly scene \\

\midrule

Spatial & Spatial 2D &
A black cat sitting \hlkw{to the left of a red suitcase} on the floor inside an airport terminal, soft indoor lighting \\

Spatial & Spatial 3D &
A drone flying \hlkw{high above a forest valley} with mountains in the distance and mist in the air, aerial cinematic photography \\

Spatial & Relative Position &
A coffee cup placed \hlkw{behind a laptop} on a wooden desk with scattered notebooks and pens, cozy workspace lighting \\

Spatial & Perspective &
A busy city street viewed \hlkw{from a high rooftop looking down} at traffic and pedestrians, dramatic perspective, night lights \\

\midrule

Relations & Object Interaction &
A child \hlkw{throwing a ball to a dog} in a green park with trees and sunshine, action moment captured, natural lighting \\

Relations & Comparative Relation &
A \hlkw{tall giraffe standing next to a shorter zebra} in an African savanna landscape during golden hour \\

Relations & Multi Relation &
A \hlkw{man handing a book to a woman while a child watches} in a library filled with bookshelves and warm lighting \\

\bottomrule
\end{tabularx}
\label{tab:prompt_cat_3}
\end{table}

\begin{table}[!t]
\centering
\caption{Illustrative prompts from the \grayhl{\textbf{\textit{Actions}}}, \grayhl{\textit{\textbf{Scene Understanding}}}, and \grayhl{\textit{\textbf{Text and Symbols}}} semantic dimensions, continuing Tab.~\ref{tab:prompt_cat_3}. Words or phrases corresponding to each subcategory within these dimensions are highlighted for clarity.}
\footnotesize
\begin{tabularx}{\textwidth}{p{3.6cm} p{3.6cm} >{\raggedright\arraybackslash}X}
\toprule
\textbf{Prompt Category} & \textbf{Subcategory} & \textbf{Prompt Example} \\
\midrule

Actions & Human Action &
A chef \hlkw{chopping vegetables} on a kitchen counter with knives and ingredients spread around, culinary action photography \\

Actions & Animal Action &
A cat \hlkw{jumping from a chair onto a wooden table} inside a bright kitchen, motion captured mid-air \\

Actions & Object Manipulation &
A robotic arm \hlkw{assembling a smartphone} on a futuristic factory assembly line, glowing lights, advanced technology scene \\

\midrule

Scene Understanding & Indoor Scene &
A \hlkw{cozy living room interior} with sofa, lamp, bookshelf, and soft warm lighting, realistic interior photography \\

Scene Understanding & Outdoor Scene &
People walking through a \hlkw{busy outdoor street market} with colorful stalls, fruits, fabrics, and vibrant atmosphere \\

Scene Understanding & Urban Scene &
A \hlkw{dense urban city skyline} filled with skyscrapers and busy traffic during sunset, cinematic lighting, ultra detailed \\

Scene Understanding & Natural Scene &
A \hlkw{calm lake surrounded by pine trees and mountains} reflecting in the water during sunrise, peaceful natural landscape \\

\midrule

Text and Symbols & Text in Image &
A street sign clearly displaying the word \hlkw{STOP} in bright red letters at a city intersection \\

Text and Symbols & Symbol Rendering &
A glowing neon \hlkw{peace symbol} mounted on a dark brick wall in a nighttime urban alley \\

Text and Symbols & Logo or Sign &
High quality simplified rectangular \hlkw{logo of a medieval stone blacksmith forge} shaped like a realistic dragon head looking at viewer, for a company called poly - forge, symmetrical!!!, award winning, art deco!!!!!! by milton glaser \\

\bottomrule
\end{tabularx}
\label{tab:prompt_cat_4}
\end{table}

\begin{table}[!t]
\centering
\caption{Illustrative prompts from the \grayhl{\textbf{\textit{Style and Aesthetics}}} semantic dimension, continuing Tab.~\ref{tab:prompt_cat_4}. Words or phrases corresponding to each subcategory within this dimension are highlighted for clarity.
}
\footnotesize
\begin{tabularx}{\textwidth}{p{3.6cm} p{3.6cm} >{\raggedright\arraybackslash}X}
\toprule
\textbf{Prompt Category} & \textbf{Subcategory} & \textbf{Prompt Example} \\
\midrule

Style and Aesthetics & Art Style &
A heroic warrior portrait illustrated in \hlkw{medieval fantasy art style}, detailed armor, dramatic lighting, epic composition \\

Style and Aesthetics & Photographic Style &
A professional \hlkw{portrait photograph} of a woman with soft lighting and shallow depth of field, studio photography \\

Style and Aesthetics & Artist Style &
A portrait painting of a woman in the style of \hlkw{Vincent van Gogh} with expressive brush strokes and vivid colors \\

Style and Aesthetics & Genre Style &
A retro \hlkw{science fiction poster} showing a spaceship flying over a futuristic city in bold 1980s illustration style \\

Style and Aesthetics & Surreal Scene &
A \hlkw{surreal floating island} in the sky with upside down waterfalls and glowing crystals, fantasy concept art \\

Style and Aesthetics & Anti-realism &
A \hlkw{rhombohedral, cubist} small pink square with an irregular diagonal, and white triangle above it by jacques villon, trending on flickr, crystal cubism, angular, cubism, geometric. \\

Style and Aesthetics & Fantasy Content &
A \hlkw{dragon flying over a castle} during a stormy night, lightning in the sky, epic fantasy digital painting \\

\bottomrule
\end{tabularx}
\label{tab:prompt_cat_5}
\end{table}

\clearpage
\section{Model Tiering}
\label{supp:mt}

Tab.~\ref{tab:dyneval_models} reports the complete ranking of the \textbf{36} T2I models considered in DynEval, along with their DynEval scores and corresponding tier assignments. Following \cref{sec:gendb} of the main paper, each T2I model is evaluated on the DynEval-1K evaluation set by averaging the teacher model's predicted DynEval scores over 1,000 generated prompt-image pairs. Based on these scores, the models are partitioned into three capability tiers using two empirically selected thresholds ($\mu_1$ and $\mu_2$), where Tier-1 denotes the strongest models and Tier-3 the weakest. The proposed tiering serves two complementary purposes. First, it enables the \textit{tier-matched prompt-model generation} strategy adopted during GenDB construction, where Tier-1, Tier-2, and Tier-3 models are paired with hard, medium, and easy prompts, respectively. Since weaker models often struggle even with simpler prompts whereas stronger models rarely fail on easier prompts, matching model capability with prompt complexity results in a broader and more diverse set of semantic and perceptual failure cases. Second, the tier assignments facilitate the fine-grained analysis of model capabilities presented in \cref{fig:category_score} of the main paper by additionally comparing the best-performing (Fig.~\ref{fig:category_score_best}) and worst-performing (Fig.~\ref{fig:category_score_worst}) models from each tier across the 42 prompt subcategories.

On the DynEval-1K evaluation set, Tier-1, Tier-2, and Tier-3 models achieve average DynEval scores of $0.872 \pm 0.041$, $0.739 \pm 0.039$, and $0.528 \pm 0.123$, respectively. The tier thresholds are selected empirically by analyzing the score distribution in Tab.~\ref{tab:dyneval_models}; specifically, we define two thresholds, $\mu_1$ and $\mu_2$ ($\mu_1 > \mu_2$), and set them to \textbf{0.81} and \textbf{0.67}, respectively. Notably, these thresholds should be interpreted as relative groupings rather than universal performance boundaries, since different prompt distributions or T2I model pools would naturally produce different score distributions and, consequently, different threshold values.
\begin{table}[!t]
\centering

\caption{
\textbf{Overall performance of 36 T2I models on the DynEval-1K evaluation set.} Models are ordered according to the teacher model's predicted DynEval score (normalized to $[0,1]$) and grouped into three capability tiers. We also report the mean and standard deviation of each tier.
}

\footnotesize
\vspace{-2mm}
\setlength{\tabcolsep}{7pt}
\begin{tabular}{l | c | c |c}
\toprule
\textbf{Model} & \textbf{Tier} & \textbf{DynEval Score} & \textbf{Avg $\pm$ Std} \\
\midrule

GPT-Image-1.5~\cite{gpt_image_1_5} & \multirow{7}{*}{TIER-1} & 0.934 & \multirow{7}{*}{0.872 $\pm$ 0.041} \\
NanoBanana~\cite{team2023gemini} & & 0.915 & \\
FLUX.2 [klein]~\cite{flux-2-2025} & & 0.883 & \\
FLUX.2 [dev]~\cite{flux-2-2025} & & 0.866 & \\
FIBO~\cite{gutflaish2025generating} & & 0.844 & \\
LongCat-Image~\cite{LongCat-Image} & & 0.834 & \\
HiDream-I1~\cite{hidreami1technicalreport} & & 0.830 & \\

\midrule

Qwen-Image~\cite{wu2025qwen} & \multirow{19}{*}{TIER-2} & 0.793 & \multirow{19}{*}{0.739 $\pm$ 0.039} \\
Z-Image~\cite{team2025zimage} & & 0.789 & \\
GLM-Image~\cite{glmimage2024} & & 0.780 & \\
FLUX.1 [dev]~\cite{labs2025flux1kontextflowmatching} & & 0.776 & \\
Sana~\cite{xie2024sana} & & 0.769 & \\
UniPic~\cite{wang2025skywork} & & 0.768 & \\
Stable Diffusion 3.5~\cite{esser2024scaling} & & 0.767 & \\
OmniGen2~\cite{wu2025omnigen2} & & 0.765 & \\
In-Context LoRA~\cite{huang2024context} & & 0.757 & \\
Bagel~\cite{deng2025bagel} & & 0.755 & \\
OmniGen~\cite{xiao2025omnigen} & & 0.741 & \\
Hunyuan-DiT~\cite{li2024hunyuan_dit} & & 0.727 & \\
Show-o~\cite{xie2024show} & & 0.711 & \\
X-Omni~\cite{geng2025x} & & 0.706 & \\
Janus-Pro~\cite{chen2025janus} & & 0.696 & \\
Kolors~\cite{kolors} & & 0.689 & \\
PixArt-$\alpha$~\cite{chen2023pixart} & & 0.685 & \\
Kandinsky 3~\cite{arkhipkin2023kandinsky} & & 0.683 & \\
UniWorld-V1~\cite{lin2025uniworld} & & 0.682 & \\

\midrule

Playground v2.5~\cite{li2024playground} & \multirow{10}{*}{TIER-3} & 0.655 & \multirow{10}{*}{0.528 $\pm$ 0.123} \\
SSD-1B~\cite{gupta2024progressive} & & 0.613 & \\
DeepFloyd IF-XL~\cite{deepfloydif2023} & & 0.609 & \\
Emu3~\cite{wang2024emu3} & & 0.597 & \\
SDXL-Turbo~\cite{podell2023sdxl} & & 0.594 & \\
Stable Diffusion XL~\cite{podell2023sdxl} & & 0.553 & \\
Stable Diffusion v2.1~\cite{rombach2022high} & & 0.523 & \\
Stable Diffusion v1.5~\cite{rombach2022high} & & 0.475 & \\
PixArt-$\Sigma$~\cite{chenweak} & & 0.425 & \\
LlamaGen~\cite{sun2024autoregressive} & & 0.240 & \\

\bottomrule
\end{tabular}

\label{tab:dyneval_models}
\vspace{-5mm}
\end{table}

\section{Details on Tier-Specific Thresholds}
\label{supp:tst}

As described in \cref{sec:gendb} of the main paper, GenDB is constructed using the proposed \textit{tier-matched prompt-model pairing} strategy. Building upon GenDB, \cref{sec:DynEvalInstruct} introduces a second-stage curation process to construct DynEvalInstruct using teacher-generated T2IA and IQA responses. For each prompt-image pair, the T2IA and IQA scores are obtained from the teacher model's responses and combined into a single scalar score: $S = 0.5 \times S_{\mathrm{T2IA}} + 0.5 \times S_{\mathrm{IQA}}$. Since GenDB contains images generated by three T2I model tiers with different performance ranges, the curation framework employs tier-specific selection thresholds $\delta_i$, where $i \in \{1,2,3\}$. A sample generated by a Tier-$i$ model is retained if $S < \delta_i$. In practice, we found that a common threshold was sufficient across all tiers and therefore set $\delta_1 = \delta_2 = \delta_3 = 5$. Since the maximum possible combined score is $S=5$, this criterion removes only prompt-image pairs that receive the highest possible score. Such samples typically exhibit near-perfect text-image alignment and visual quality, providing limited supervision for learning fine-grained evaluator behavior. Consequently, we retain only samples satisfying $S<5$, which are more likely to contain semantic, compositional, or perceptual discrepancies that serve as informative training examples. Applying this filtering strategy to GenDB yields the final 250K-sample DynEvalInstruct dataset. Notably, as shown in Sec.~\ref{supp:data_scaling}, evaluator performance begins to saturate at approximately 250K training samples, with only marginal improvements beyond this point.
\section{Additional Ablation Study}
\label{supp:aas}

\begin{wraptable}[15]{r}{0.6\textwidth}
\vspace{-12mm}
\centering
\caption{\textbf{Ablation on teacher model selection.} Average DynEval score (mean $\pm$ standard deviation) for different teacher model candidates evaluated on the DynEval-1K evaluation set. Scores are normalized to the range $[0,1]$. Lower scores correspond to stricter evaluators and are therefore preferred for knowledge distillation.}
\label{tab:teacher_ablation}

\small
\resizebox{0.6\columnwidth}{!}{%
\begin{tabular}{lc}
\toprule
\textbf{Model} & \textbf{DynEval Score} ($\downarrow$) \\
\midrule

Qwen3-VL-235B-A22B-Instruct~\cite{Bai2025qwen} & $0.850 \pm 0.192$ \\
GPT-5.1~\cite{gpt51_openai_2025} & $0.863 \pm 0.216$ \\
InternVL3.5-241B-A28B~\cite{wang2025internvl3}  & $0.900 \pm 0.100$ \\
InternVL3-78B~\cite{zhu2025internvl3} & $0.920 \pm 0.084$ \\
Qwen3-VL-32B-Instruct~\cite{Bai2025qwen} & $0.929 \pm 0.076$ \\
Qwen3-VL-8B-Instruct~\cite{Bai2025qwen} & $0.971 \pm 0.076$ \\
\bottomrule
\end{tabular}}
\vspace{-8pt}
\end{wraptable}
\subsection{Teacher Model Selection}
\label{supp:teacher_choice}
While \cref{tab:main_comp} in the main paper presents the student model ablation, here we provide additional ablations on the teacher model selection and investigate the effect of data scaling during fine-tuning. In Tab.~\ref{tab:teacher_ablation}, we report the average scores of different teacher model candidates evaluated on the DynEval-1K evaluation set. As a text-to-image evaluator, the teacher model should ideally adopt a stricter perspective, penalizing generated images when necessary and assigning lower scores accordingly. From Tab.~\ref{tab:teacher_ablation}, we observe that \texttt{Qwen3-VL-235B}~\cite{Bai2025qwen} best satisfies this criterion and is therefore the most suitable teacher model for distillation.

\subsection{Training Data Scaling}
\label{supp:data_scaling}

\begin{wraptable}[18]{r}{0.36\textwidth}
\vspace{-12mm}
\centering
\caption{\textbf{Ablation on training data scaling.} Performance of the DynEval-4B evaluator trained with different amounts of DynEvalInstruct data, evaluated using SRCC (mean $\pm$ standard deviation) on the TIFA~\cite{tifa} dataset. Scores are normalized to the range $[0,1]$. Correlation with human judgments improves consistently with increasing training set size and begins to saturate at approximately 250K training samples.}
\label{tab:data_scaling}

\small
\resizebox{0.35\columnwidth}{!}{%
\begin{tabular}{cc}
\toprule
\textbf{Training Data} & \textbf{SRCC} ($\uparrow$) \\
\midrule
50K  & $0.687 \pm 0.023$ \\
100K & $0.700 \pm 0.018$ \\
150K & $0.750 \pm 0.007$ \\
200K & $0.790 \pm 0.010$ \\
250K & $0.800 \pm 0.003$ \\
\bottomrule
\end{tabular}}
\vspace{-8pt}
\end{wraptable}
Tab.~\ref{tab:data_scaling} presents the training data scaling ablation for our DynEval-4B evaluator. As the size of the DynEvalInstruct training data increases from 50K to 250K samples, the Spearman Rank Correlation Coefficient (SRCC) with human judgments improves consistently, demonstrating the effectiveness of scaling supervision without relying on human-annotated data. Notably, performance begins to saturate at approximately 250K training samples, indicating diminishing returns beyond this point.
\section{Additional Qualitative Results}
\label{supp:added_visual_results}

\begin{figure}[!t]
    \centering
    \includegraphics[width=\linewidth]{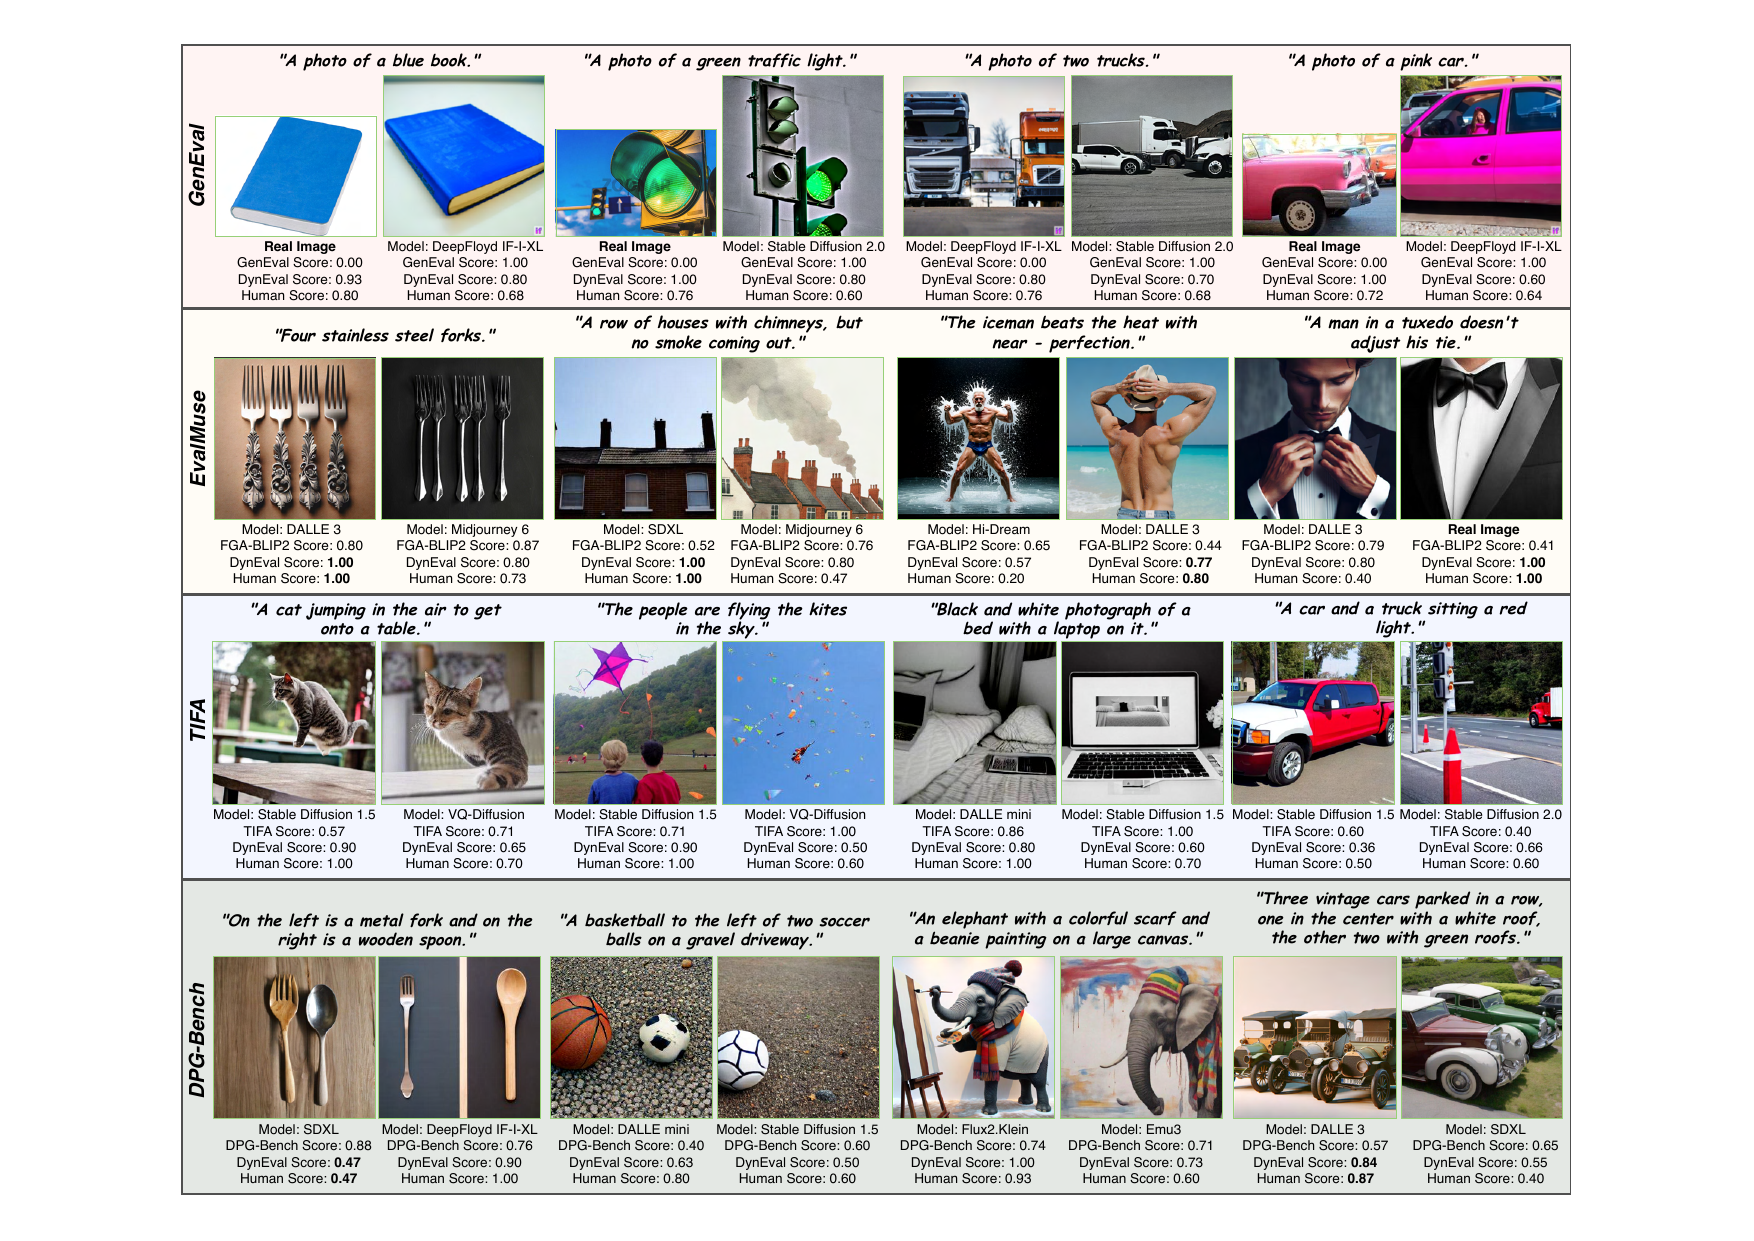}
    \vspace{-6mm}
    \caption{
    \textbf{Additional qualitative comparisons extending \cref{fig:qualitative_comp} in the main paper.} Comparison of DynEval-4B with representative T2I evaluation methods, including GenEval~\cite{GenEval}, TIFA~\cite{tifa}, DPG-Bench~\cite{DPGBench}, and EvalMuse~\cite{EvalMuse-40k}, together with human ratings. All scores are normalized to the range $[0,1]$ for fair comparison. The examples highlight representative failure cases of existing T2I evaluators, including detector dependency (GenEval~\cite{GenEval}), inaccurate semantic scoring (TIFA~\cite{tifa} and DPG-Bench~\cite{DPGBench}), and difficulties with negation and counting (EvalMuse~\cite{EvalMuse-40k}), while demonstrating that DynEval consistently produces scores that more closely align with human judgments by jointly evaluating text-image alignment and image quality.}
    \label{fig:supp_teaser_fig}
    \vspace{-5mm}
    
\end{figure}

In Fig.~\ref{fig:supp_teaser_fig}, we present additional qualitative comparisons that extend \cref{fig:qualitative_comp} from the main paper between DynEval and four representative T2I evaluation methods: GenEval~\cite{GenEval}, TIFA~\cite{tifa}, DPG-Bench~\cite{DPGBench}, and EvalMuse~\cite{EvalMuse-40k}. For a fair visual comparison, the scores from all evaluators, together with the human ratings, are normalized to the range $[0,1]$. GenEval~\cite{GenEval} evaluates object-centric compositional properties such as object presence, object count, color, and spatial relationships by leveraging an object detection model together with CLIP~\cite{radford2021learning}. However, because it relies heavily on the performance of the underlying object detector, it often fails to detect the presence of an object even when it is clearly visible in both the real and generated images, as illustrated in Fig.~\ref{fig:supp_teaser_fig}. This detector-dependent design limits GenEval's evaluation capability. TIFA~\cite{tifa} extends this paradigm through prompt-derived VQA-based T2I assessment, while DPG-Bench~\cite{DPGBench} emphasizes dense prompts involving multiple objects, attributes, and relationships by leveraging DSG~\cite{cho2023davidsonian}. However, these two approaches focus only on evaluating semantic alignment and do not explicitly account for perceptual image quality, resulting in two major contradictions: (i) visually superior images may receive disproportionately low scores, and (ii) visually distorted or semantically implausible images may receive overly high scores, as shown in Fig.~\ref{fig:supp_teaser_fig}. EvalMuse~\cite{EvalMuse-40k} further improves alignment evaluation through fine-grained prompt decomposition and the training of a T2I evaluator using 40K human-annotated ratings. However, the resulting evaluator often struggles with negation prompts and counting tasks involving multiple objects, as depicted in Fig.~\ref{fig:supp_teaser_fig}, highlighting the need for large-scale prompt exposure during evaluator training. In contrast, DynEval jointly evaluates text-image alignment (T2IA) and image quality assessment (IQA), enabling it to distinguish images with similar semantic correctness but substantially different visual quality. Trained on 250K samples without relying on human annotations, DynEval produces scores that more closely follow human judgments across the diverse examples shown in Fig.~\ref{fig:supp_teaser_fig}, often matching the human score exactly.
\section{Understanding Failure Attributes of T2I Models}
\label{supp:failure}

\cref{fig:category_score} of the main paper reports the average DynEval-4B predicted scores for Tier-1, Tier-2, and Tier-3 models across all 42 prompt subcategories in the DynEval-1K evaluation set. While these averages provide a high-level comparison across the three tiers, they do not capture the variability among models within the same tier. To better understand this intra-tier variation, Fig.~\ref{fig:category_score_best} and Fig.~\ref{fig:category_score_worst} present the highest-scoring and lowest-scoring models from each tier across all prompt subcategories. Specifically, \texttt{GPT-Image-1.5}, \texttt{Qwen-Image}~\cite{wu2025qwen}, and \texttt{Playground v2.5}~\cite{li2024playground} emerge as the best-performing models in Tier-1, Tier-2, and Tier-3, respectively, as shown in Fig.~\ref{fig:category_score_best}. Although these models exhibit consistently strong performance across most semantic dimensions, they show noticeable performance degradation on certain subcategories. Moreover, Fig.~\ref{fig:category_score_worst} highlights the weakest-performing model within each tier, revealing substantially lower performance across nearly all semantic dimensions. For example, \texttt{LlamaGen}~\cite{sun2024autoregressive}, the weakest Tier-3 model, consistently struggles with both object-centric prompts and more challenging compositional reasoning tasks. Nevertheless, the considerable performance gap between the best-performing and worst-performing models does not alter the relative ordering of the most challenging prompt categories, which remains remarkably consistent across all tiers. Notably, subcategories such as \textit{human present}, \textit{count multi objects}, \textit{size binding}, \textit{perspective}, \textit{anti-realism}, and \textit{text in image} remain among the lowest-scoring subcategories regardless of overall model strength, indicating that these semantic capabilities continue to be challenging for current T2I models.

Overall, these results demonstrate that the proposed tier assignments effectively capture broad differences in model capability while preserving meaningful variation among models within the same tier. They also show that models with comparable overall DynEval scores can still exhibit distinct strengths and weaknesses across individual semantic dimensions, motivating fine-grained category-wise analysis in addition to overall benchmark performance.

\begin{figure}[!t]
    \centering
    \includegraphics[width=\linewidth]{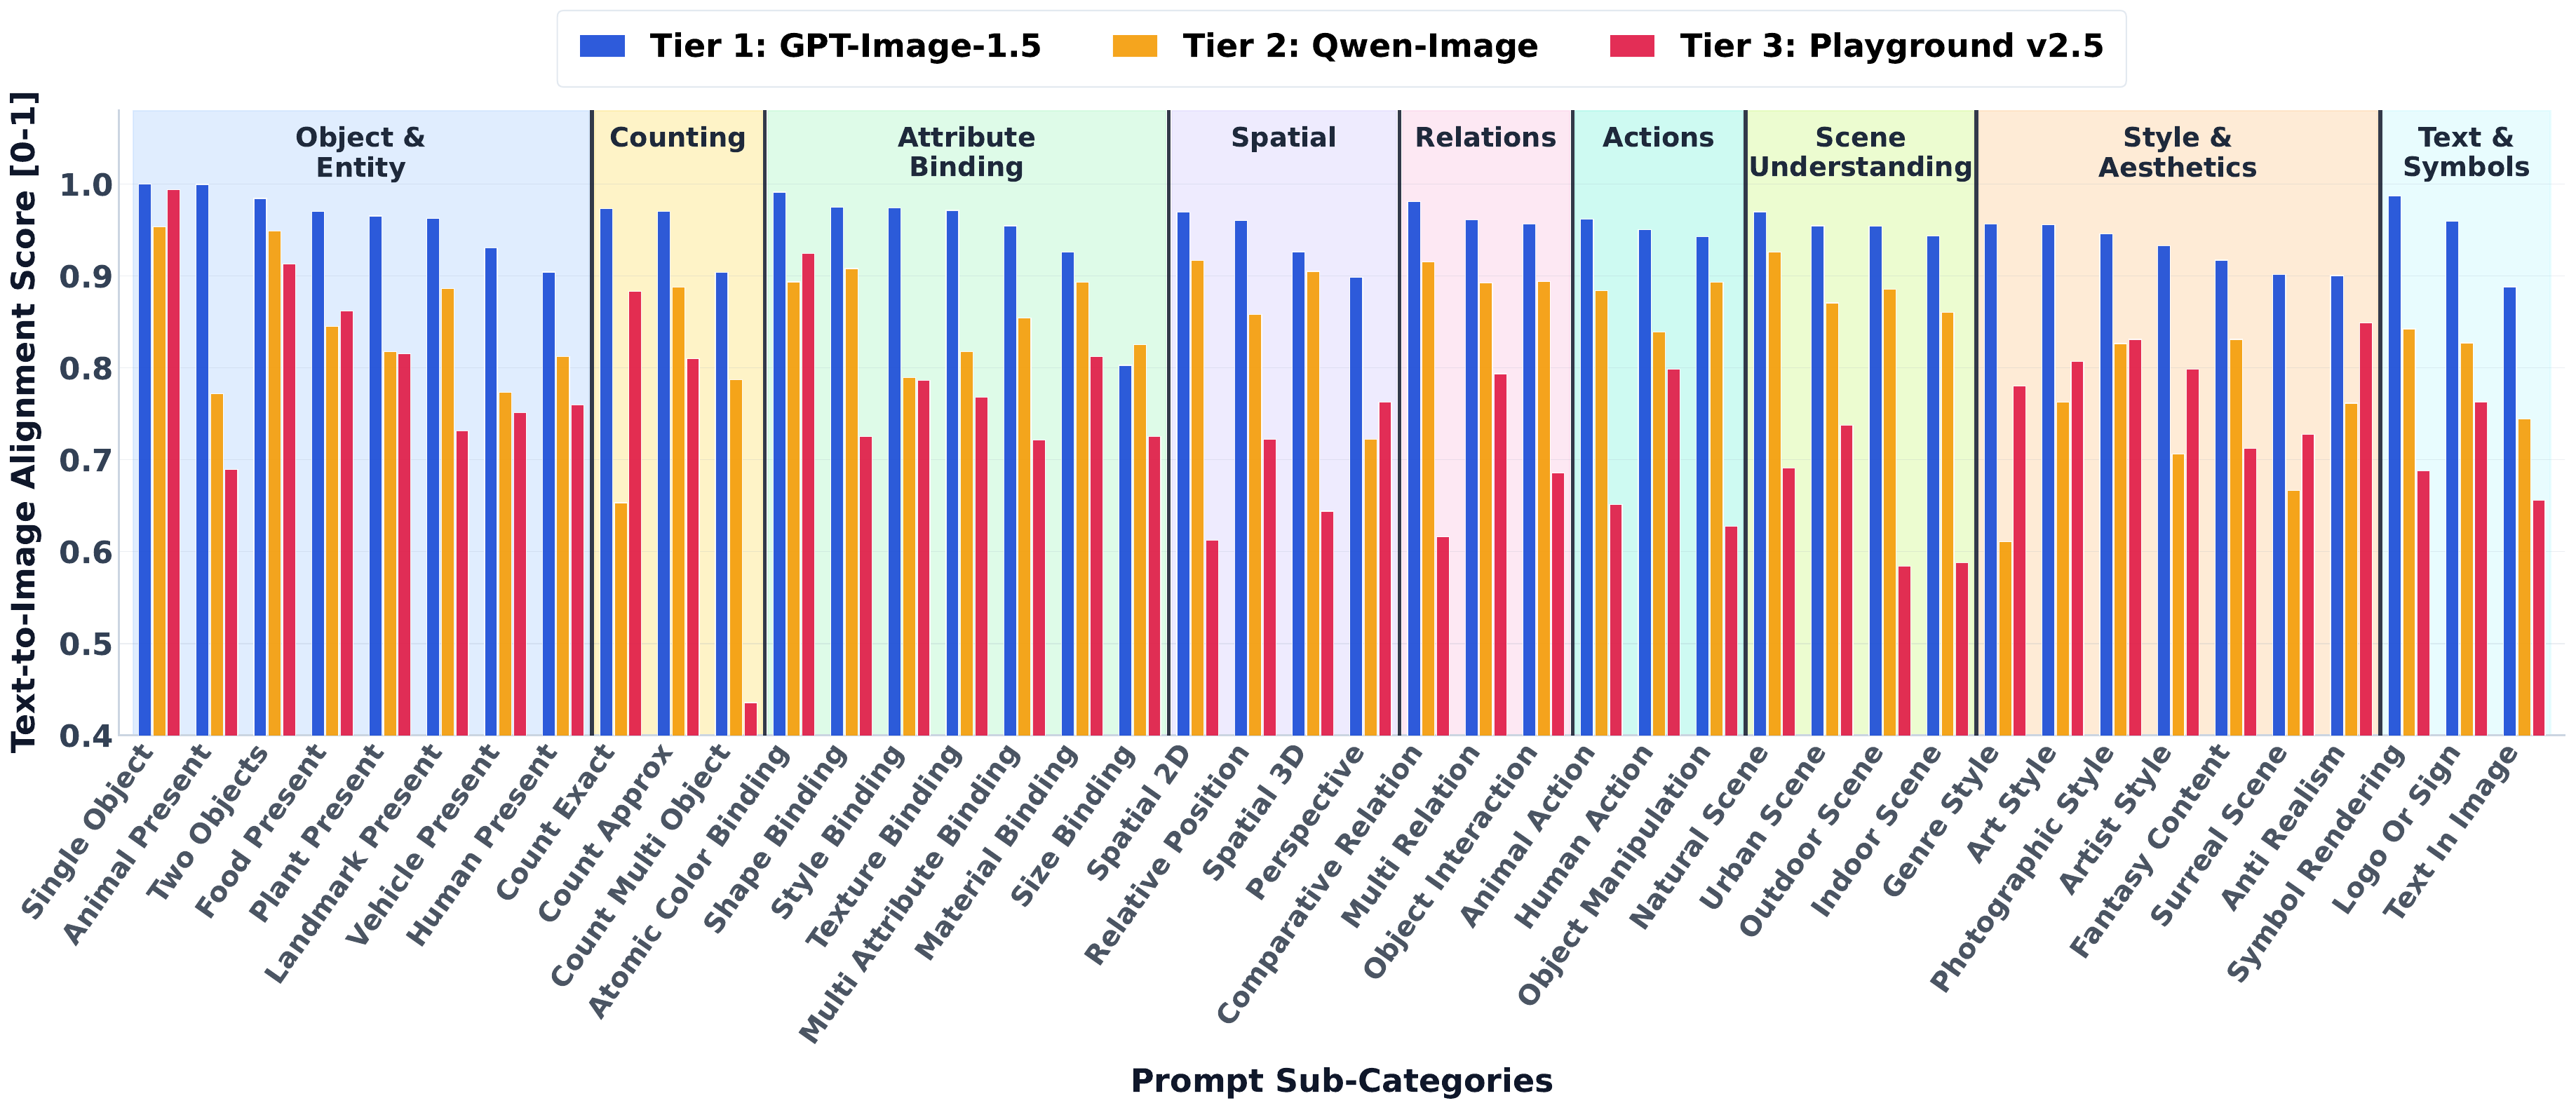} 
    \caption{Performance of the \textbf{best-scoring model} from each model tier across the 42 prompt subcategories on the \textbf{DynEval-1K} evaluation set. GPT-Image-1.5~\cite{gpt_image_1_5}, Qwen-Image~\cite{wu2025qwen}, and Playground v2.5~\cite{li2024playground} are the highest-ranked models in Tier-1, Tier-2, and Tier-3, respectively, based on their DynEval-4B predicted scores. Although these models achieve consistently strong performance across most semantic dimensions, they continue to exhibit noticeable weaknesses on challenging subcategories such as \textit{human present}, \textit{count multi objects}, \textit{size binding}, \textit{perspective}, \textit{anti-realism}, and \textit{text in image}.}
    \label{fig:category_score_best}
\end{figure}

\begin{figure}[!t]
    \centering
    \includegraphics[width=\linewidth]{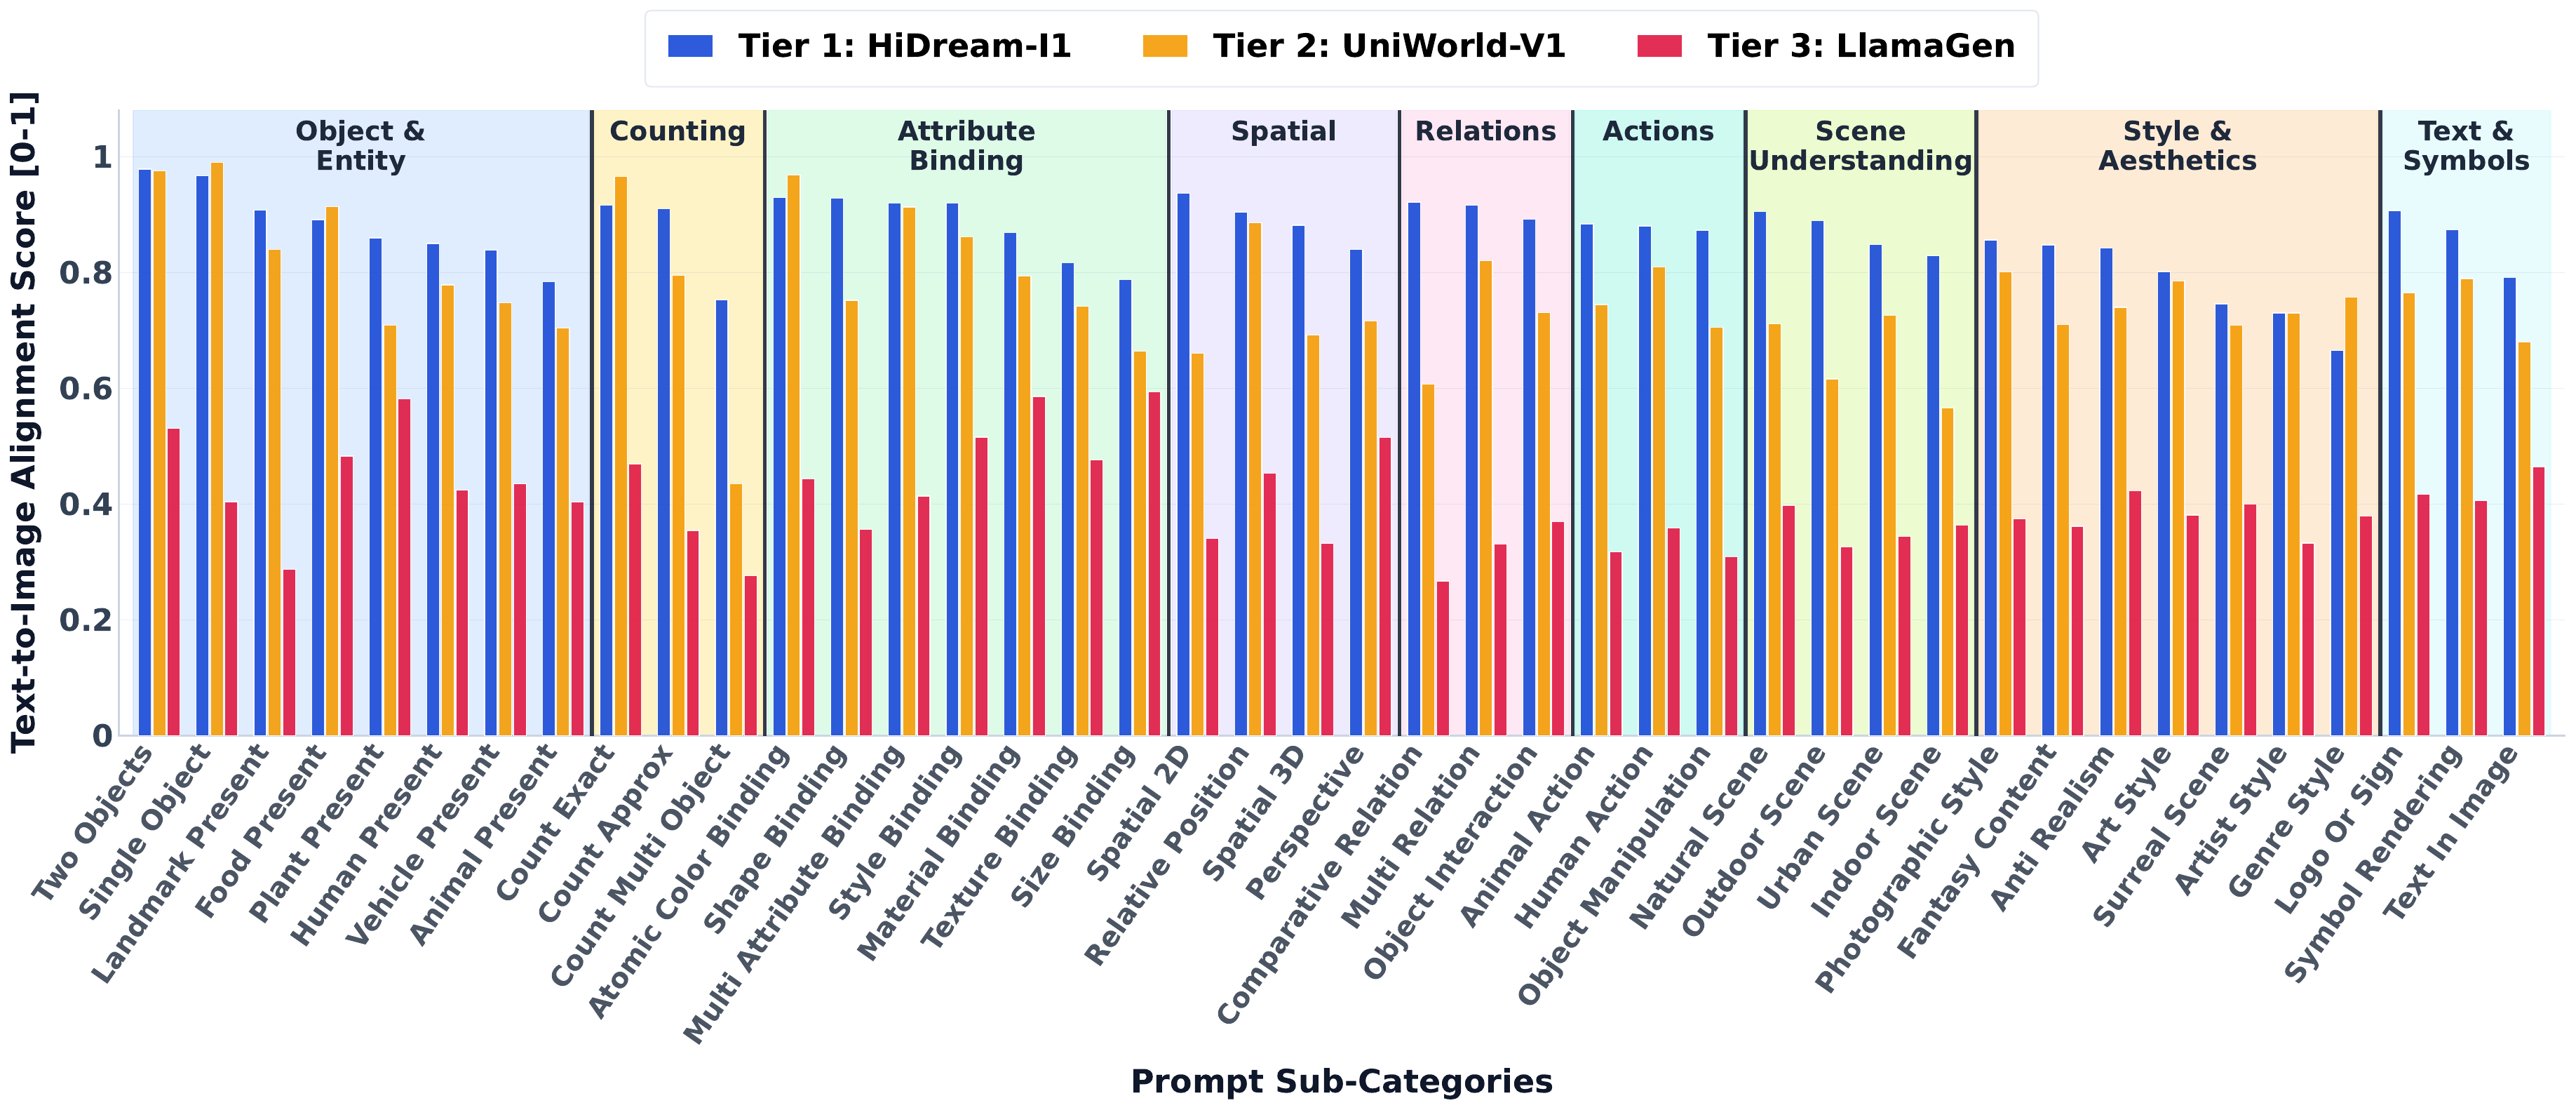}
    \caption{Performance of the \textbf{lowest-scoring model} from each model tier across the 42 prompt subcategories on the \textbf{DynEval-1K} evaluation set. HiDream-I1~\cite{hidreami1technicalreport}, UniWorld-V1~\cite{lin2025uniworld}, and LlamaGen~\cite{sun2024autoregressive} are the lowest-ranked models in Tier-1, Tier-2, and Tier-3, respectively, based on their DynEval-4B predicted scores. These models exhibit substantially lower performance across nearly all semantic dimensions, while the relative ordering of the most challenging prompt subcategories remains largely consistent across all model tiers.}
    \label{fig:category_score_worst}
    \vspace{-5mm}
\end{figure}
