# Supplementary material for: DynEval: Holistic Evaluations of T2I Generative Models in the Wild
Source: arXiv:2607.11199 source file (2026-07-13)
Supplement: Supplementary file 2 [file 1_benchmark_details.tex]

\section{Benchmark Dataset Details}
\label{supp:dataset_Details}

\begin{table*}[t]
\centering
\caption{
\textbf{Statistics of existing T2I evaluation benchmarks.} \grayhl{\textbf{\#Prompts}} denotes the number of unique prompts, \grayhl{\textbf{\#Pairs}} the total number of image-text pairs, \grayhl{\textbf{Images/T2I}} the average number of images contributed by each T2I generative model, and \grayhl{\textbf{\#T2I}} the total number of T2I models evaluated in each benchmark. For \grayhl{\textbf{Prompt Length}}, we report the minimum, maximum, and mean $\pm$ standard deviation ($\mu \pm \sigma$), computed over the number of characters in each prompt, including whitespace and punctuation. \textbf{Mixed} in the \textbf{Images/T2I} column indicates that the number of images contributed by each model varies; therefore, a single images-per-model value cannot be reported. The blank entry for RichHF in the \textbf{Images/T2I} column indicates that RichHF does not provide T2I model metadata for the generated images; therefore, a per-model image count cannot be reported.
}
\label{tab:benchmark_statistics}
\vspace{-3mm}
\small
\setlength{\tabcolsep}{5pt}
\resizebox{\textwidth}{!}{
\begin{tabular}{r|l|l|l|l|l|l|r}
\toprule
\multirow{2}{*}{\textbf{Benchmark}} &
\multirow{2}{*}{\textbf{\#Prompts}} &
\multirow{2}{*}{\textbf{\#Pairs}} &
\multicolumn{3}{c|}{\textbf{Prompt Length}} &
\multirow{2}{*}{\textbf{Images/T2I}} &
\multirow{2}{*}{\textbf{\#T2I}} \\
\cmidrule(lr){4-6}
& & &
\textbf{Min} &
\textbf{Max} &
\textbf{$\mu \pm \sigma$} &
& \\
\midrule
T2I-CoReBench~\cite{T2I-CoReBench}   & 1,080 & 4,320  & 238 & 2,064 & 764.62 $\pm$ 324.51 & 1,080 & 4 \\
TIIF-Bench~\cite{tiff_bench} & 529   & 2,216  & 27  & 2,478 & 358.75 $\pm$ 387.44 & 554   & 4 \\
UniGenBench++~\cite{unigenbench++} & 600   & 3,587  & 64  & 300   & 158.60 $\pm$ 33.81  & Mixed & 6 \\
LMM4LMM~\cite{lmm4lmm_evalmi-50k} & 2,086 & 10,080 & 16  & 1,876 & 98.26 $\pm$ 145.32  & 420   & 24 \\
RichHF~\cite{liang2024rich} & 493   & 955    & 4   & 1,018 & 79.31 $\pm$ 110.69  & --    & 3 \\
EvalMuse~\cite{EvalMuse-40k}        & 989   & 10,796 & 6   & 335   & 68.62 $\pm$ 45.04   & Mixed & 20 \\
GenAI-Bench~\cite{li2024genai}     & 1,600 & 9,600  & 14  & 192   & 67.42 $\pm$ 26.89   & 1,600 & 6 \\
TIFA~\cite{tifa} & 160   & 800    & 13  & 182   & 56.13 $\pm$ 26.90   & 160   & 5 \\
T2I-Eval-Bench~\cite{t2i_eval_bench}  & 8,772 & 8,772  & 25  & 217   & 54.19 $\pm$ 12.54   & Mixed & 3 \\
GenEval 2~\cite{geneval2}        & 800   & 3,200  & 13  & 93    & 50.82 $\pm$ 18.41   & 800   & 4 \\
GenEval~\cite{GenEval} & 100   & 1,200  & 16  & 54    & 31.19 $\pm$ 9.46    & 400   & 3 \\
\bottomrule
\end{tabular}
}
\vspace{-2mm}
\end{table*}

\myparagraph{\textit{Benchmark Dataset Statistics.}} We evaluate \textbf{DynEval} on a diverse collection of 11 text-to-image (T2I) evaluation benchmarks spanning: \textbf{(i)} attribute binding, counting, and spatial relations (GenEval~\cite{GenEval}, GenEval2~\cite{geneval2}, TIFA~\cite{tifa}, and GenAI-Bench~\cite{li2024genai}); \textbf{(ii)} long-form instruction following and complex multi-object interactions (TIIF-Bench~\cite{tiff_bench} and UniGenBench++~\cite{unigenbench++}); \textbf{(iii)} text and symbol rendering (TIIF-Bench~\cite{tiff_bench} and EvalMi~\cite{lmm4lmm_evalmi-50k}); \textbf{(iv)} complex compositional understanding and reasoning (T2I-CoReBench~\cite{T2I-CoReBench}); and \textbf{(v)} human preference evaluations (RichHF~\cite{liang2024rich}). These benchmarks cover a broad spectrum of challenges encountered in modern T2I evaluation, thereby providing complementary testbeds for assessing the robustness and generalization of automatic T2I evaluators. \cref{tab:benchmark_statistics} summarizes the corresponding benchmark statistics, including dataset scale, prompt length, and coverage of T2I models. Specifically, the number of unique prompts ranges from 100 (GenEval~\cite{GenEval}) to 8,772 (T2I-Eval-Bench~\cite{t2i_eval_bench}), while the number of image-text pairs varies from 800 (TIFA~\cite{tifa}) to 10,796 (EvalMuse~\cite{EvalMuse-40k}). Furthermore, prompt complexity varies considerably across benchmarks: the average prompt length ranges from $31.19$ in GenEval~\cite{GenEval} to $764.62$ in T2I-CoReBench~\cite{T2I-CoReBench}, reflecting the recent trend toward increasingly long and semantically complex prompts. In our analysis, prompt length is measured as the number of characters in each prompt, including whitespace and punctuation. Likewise, the number of generated images per T2I model and the number of evaluated models vary substantially across benchmarks, with the latter ranging from 3 to 24 models. Collectively, these statistics demonstrate that our evaluation encompasses a diverse range of benchmark characteristics, enabling a comprehensive assessment of \textbf{DynEval}'s robustness and generalization across varying prompt complexities and image generation scenarios.

\myparagraph{\textit{Human Annotations.}} As noted in the main paper, GenEval2~\cite{geneval2}, TIIF-Bench~\cite{tiff_bench}, UniGenBench++~\cite{unigenbench++}, and T2I-CoReBench~\cite{T2I-CoReBench} do not provide publicly available human annotations. Moreover, GenEval2~\cite{geneval2} does not release the images used in its evaluation protocol. To facilitate evaluation on GenEval2, we generate images for its 800 evaluation prompts using four recent text-to-image generative models, namely GPT-Image-1.5~\cite{gpt_image_1_5}, NanoBanana~\cite{team2023gemini}, Qwen-Image~\cite{wu2025qwen}, and FLUX.2 [dev]~\cite{flux-2-2025}, resulting in 3,200 prompt-image pairs. We then collect human annotations for all four benchmarks using a unified annotation protocol. Since our objective is to evaluate both text-to-image alignment (T2IA) and image quality assessment (IQA), we adopt an attribute-centric annotation strategy inspired by EvalMuse~\cite{EvalMuse-40k}. Specifically, for each prompt-image pair, we decompose the input prompt into a set of atomic semantic attributes. Annotators are then presented with the prompt, the generated image, and the complete set of semantic attributes specified in the prompt, including objects, attributes, actions, counts, and spatial relations. For each semantic attribute, annotators assign a binary label: a score of 0 indicates that the generated image fails to satisfy the corresponding attribute, whereas a score of 1 indicates that the image successfully satisfies the attribute. This fine-grained annotation protocol enables a comprehensive assessment of semantic faithfulness while providing a principled proxy for perceptual image quality through aggregated attribute-level annotations. Finally, we compute a human score for each prompt-image pair by averaging the binary attribute labels, yielding a normalized score in the range $[0,1]$. Although multiple annotators per sample are generally preferred for improving annotation reliability, we employ a single annotator per sample due to practical resource constraints. We emphasize that the primary purpose of these annotations is not to introduce new human-annotated benchmarks, but rather to enable a rigorous evaluation of the proposed \textbf{DynEval} on recent and increasingly challenging T2I evaluation benchmarks.
