# Supplementary material for: DynEval: Holistic Evaluations of T2I Generative Models in the Wild
Source: arXiv:2607.11199 source file (2026-07-13)
Supplement: Supplementary file 3 [file 2_t2i_models.tex]

\section{Detailed Information of T2I Models}
\label{supp:model_details}

\begin{table*}[!ht]
\centering
\scriptsize
\caption{\textbf{Overview of the 36 T2I generative models used in DynEval.} The selected models span five years of progress in image generation (2022--2026), covering early diffusion models, diffusion transformers (DiTs), autoregressive image generation models, unified multimodal generative models, and recent large-scale foundation models. For each model, we report its release date (Year.Month), native image generation resolution, and the URL of its official repository or model release.}
\label{tab:t2i_models}
\vspace{-2mm}
\setlength{\tabcolsep}{3pt}

\begin{tabularx}{\textwidth}{l c r X}
\toprule
\textbf{Model} & \textbf{Release} & \textbf{Resolution} & \textbf{URL} \\
\midrule

Stable Diffusion v1.5 & 2022.01 & $512\times512$ & \url{https://huggingface.co/stable-diffusion-v1-5/stable-diffusion-v1-5} \\
Kandinsky 3           & 2022.11 & $1024\times1024$ & \url{https://github.com/ai-forever/kandinsky-3} \\
Stable Diffusion v2.1 & 2022.12 & $768\times768$   & \url{https://huggingface.co/sd2-community/stable-diffusion-2-1} \\
\midrule

SSD-1B                & 2023.01 & $1024\times1024$ & \url{https://huggingface.co/segmind/SSD-1B} \\
DeepFloyd IF-XL       & 2023.04 & $64\times64$     & \url{https://huggingface.co/DeepFloyd/IF-I-XL-v1.0} \\
Stable Diffusion XL   & 2023.07 & $1024\times1024$ & \url{https://huggingface.co/stabilityai/stable-diffusion-xl-base-1.0} \\
PixArt-$\alpha$          & 2023.09 & $1024\times1024$ & \url{https://github.com/PixArt-alpha/PixArt-alpha} \\
SDXL-Turbo            & 2023.11 & $512\times512$   & \url{https://huggingface.co/stabilityai/sdxl-turbo} \\
\midrule

Playground v2.5       & 2024.02 & $1024\times1024$ & \url{https://huggingface.co/playgroundai/playground-v2.5-1024px-aesthetic} \\
PixArt-$\Sigma$          & 2024.04 & $1024\times1024$ & \url{https://huggingface.co/PixArt-alpha/PixArt-Sigma-XL-2-1024-MS} \\
Hunyuan-DiT           & 2024.06 & $1024\times1024$ & \url{https://github.com/Tencent-Hunyuan/HunyuanDiT} \\
LlamaGen              & 2024.06 & $256\times256$   & \url{https://github.com/foundationvision/llamagen} \\
Kolors                & 2024.07 & $1024\times1024$ & \url{https://github.com/Kwai-Kolors/Kolors} \\
FLUX.1 [dev]            & 2024.08 & $1024\times1024$ & \url{https://huggingface.co/black-forest-labs/FLUX.1-dev} \\
Show-o                & 2024.08 & $256\times256$   & \url{https://github.com/showlab/show-o} \\
OmniGen               & 2024.09 & $1024\times1024$ & \url{https://github.com/vectorspacelab/omnigen} \\
Emu3                  & 2024.09 & $720\times720$   & \url{https://github.com/baaivision/emu3} \\
Stable Diffusion 3.5  & 2024.10 & $1024\times1024$ & \url{https://huggingface.co/stabilityai/stable-diffusion-3.5-large} \\
Sana                  & 2024.11 & $1024\times1024$ & \url{https://huggingface.co/Efficient-Large-Model/Sana_1600M_1024px} \\
In-Context LoRA       & 2024.12 & $1024\times1024$ & \url{https://huggingface.co/ali-vilab/In-Context-LoRA} \\
\midrule

Janus-Pro             & 2025.01 & $384\times384$   & \url{https://huggingface.co/deepseek-ai/Janus-Pro-7B} \\
HiDream-I1            & 2025.04 & $1024\times1024$ & \url{https://huggingface.co/HiDream-ai/HiDream-I1-Full} \\
Bagel                 & 2025.05 & $1024\times1024$ & \url{https://github.com/bytedance-seed/BAGEL} \\
OmniGen2              & 2025.06 & $1024\times1024$ & \url{https://github.com/VectorSpaceLab/OmniGen2} \\
UniWorld-V1           & 2025.06 & $1024\times1024$ & \url{https://github.com/PKU-YuanGroup/UniWorld/tree/main/UniWorld-V1} \\
UniPic                & 2025.07 & $1024\times1024$ & \url{https://github.com/SkyworkAI/UniPic/tree/main/UniPic-1} \\
Qwen-Image            & 2025.08 & $1328\times1328$ & \url{https://huggingface.co/Qwen/Qwen-Image} \\
X-Omni                & 2025.08 & $1024\times1024$ & \url{https://github.com/X-Omni-Team/X-Omni} \\
FLUX.2 [dev]            & 2025.11 & $1024\times1024$ & \url{https://huggingface.co/black-forest-labs/FLUX.2-dev} \\
FIBO                  & 2025.11 & $1024\times1024$ & \url{https://huggingface.co/briaai/FIBO} \\
GPT-Image-1.5         & 2025.12 & $1024\times1024$ & \url{https://developers.openai.com/api/docs/models/gpt-image-1.5} \\
LongCat-Image         & 2025.12 & $1024\times1024$ & \url{https://huggingface.co/meituan-longcat/LongCat-Image} \\
\midrule

FLUX.2 [klein]          & 2026.01 & $1024\times1024$ & \url{https://huggingface.co/black-forest-labs/FLUX.2-klein-9B} \\
GLM-Image             & 2026.01 & $1024\times1024$ & \url{https://huggingface.co/zai-org/GLM-Image} \\
Z-Image               & 2026.01 & $1024\times1024$ & \url{https://huggingface.co/Tongyi-MAI/Z-Image} \\
NanoBanana            & 2026.02 & $1024\times1024$ & \url{https://nanobanana.gg/} \\

\bottomrule
\end{tabularx}
\end{table*}

To construct \textbf{GenDB} and \textbf{DynEvalInstruct}, we consider a diverse collection of \textbf{36} text-to-image (T2I) generation models spanning five years of progress (2022 to 2026) in image generation. Our model pool covers: \textbf{(i)} \textbf{early diffusion-based models} such as Stable Diffusion~v1.5~\cite{rombach2022high}, Stable Diffusion~v2.1~\cite{rombach2022high}, Kandinsky~3~\cite{arkhipkin2023kandinsky}, and DeepFloyd IF-XL~\cite{deepfloydif2023}; \textbf{(ii) diffusion transformer (DiT)} models such as PixArt-$\alpha$~\cite{chen2023pixart}, Hunyuan-DiT~\cite{li2024hunyuan_dit}, FLUX.1 [dev]~\cite{flux2024}, FLUX.2 [dev]~\cite{flux-2-2025}, LongCat-Image~\cite{LongCat-Image}, GLM-Image~\cite{glmimage2024}, and Z-Image~\cite{team2025zimage}; \textbf{(iii) autoregressive image generation} models, including LlamaGen~\cite{sun2024autoregressive} and Show-o~\cite{xie2024show}; \textbf{(iv) unified multimodal generative models} such as OmniGen~\cite{xiao2025omnigen}, OmniGen2~\cite{wu2025omnigen2}, Emu3~\cite{wang2024emu3}, Janus-Pro~\cite{chen2025janus}, UniWorld-V1~\cite{lin2025uniworld}, UniPic~\cite{wang2025skywork}, and X-Omni~\cite{geng2025x}; \textbf{(v) recent open-source foundation models} such as Qwen-Image~\cite{wu2025qwen}; and \textbf{(vi) closed-source models} including \texttt{GPT-Image-1.5}~\cite{gpt_image_1_5} and \texttt{NanoBanana}~\cite{team2023gemini}. The complete list of models, along with their release dates, native generation resolutions, and official URLs, is provided in Tab.~\ref{tab:t2i_models}.

To estimate the generation capability of these models, we construct the \textbf{DynEval-1K} evaluation set, comprising 1,000 prompts sampled to cover 42 prompt subcategories across 9 semantic dimensions. Each T2I model generates one image per prompt, yielding 1,000 prompt-image pairs per model. We report the average DynEval-4B predicted score across these 1,000 prompt-image pairs as the overall capability score of each model in Tab.~\ref{tab:dyneval_models}.
