# Supplementary material for: DynEval: Holistic Evaluations of T2I Generative Models in the Wild
Source: arXiv:2607.11199 source file (2026-07-13)
Supplement: Supplementary file 4 [file 3_cbs.tex]

\section{Complexity Based Scoring}
\label{supp:cbs}

As described in \cref{sec:gendb} of the main paper, we sample prompts of varying complexity from the 1.8M human-written prompts available in DiffusionDB~\cite{DiffusionDB} using a \textit{heuristic scoring strategy} designed to estimate the semantic richness and compositional difficulty of a prompt. This scoring mechanism prioritizes prompts that are more likely to challenge the target T2I models. We first remove all prompts that contain fewer than 30 characters, where the character count includes alphabetic characters, numbers, spaces, and punctuation symbols. This filtering step eliminates overly short prompts that typically lack sufficient semantic content. For each remaining prompt $p$, we compute a score based on \textbf{9} factors capturing different aspects of prompt complexity: \textbf{(i)} prompt length, \textbf{(ii)} object and attribute counts, \textbf{(iii)} compositional density measured by the number of comma-separated clauses, \textbf{(iv)} artist or style attribution patterns (\emph{e.g.}, \textit{`in the style of'}, \textit{`art by'}, \textit{`inspired by'}), \textbf{(v)} technical rendering and fidelity terminology (\emph{e.g.}, rendering engines, lighting conditions, optics, and resolution cues), \textbf{(vi)} explicit detail descriptors (\emph{e.g.}, \textit{`highly detailed'}, \textit{`intricate'}, \textit{`sharp focus'}), \textbf{(vii)} high-level style keywords (\emph{e.g.}, \textit{`cyberpunk'}, \textit{`baroque'}), \textbf{(viii)} color specifications, and \textbf{(ix)} interaction or relational expressions. While prompt length is computed directly, the remaining eight semantic factors are extracted using \texttt{Qwen3-8B} as a metadata extraction model to identify the presence and count of the corresponding attributes in a given prompt. This hybrid design enables efficient extraction of higher-level semantic information while preserving the exact prompt length. After extracting the aforementioned metadata, we compute a \textit{heuristic complexity score} using a weighted linear combination of the nine factors:

\vspace{-2mm}
\begin{equation}
H(p) = \sum_{j=1}^{9} w_j f_j(p),
\vspace{-1mm}
\end{equation}
where $f_j(p)$ denotes the value of the $j$-th complexity attribute associated with prompt $p$. Specifically, $f_1(p)$ is computed directly from prompt length, whereas $f_j(p)$ for $j \in \{2,\ldots,9\}$ are derived from the metadata extracted using \texttt{Qwen3-8B}. The term $w_j$ denotes the weighting coefficient associated with the $j$-th attribute. Based on empirical observations, we found that prompt length ($f_1(p)$) and the number of objects and attributes ($f_2(p)$) are the most reliable indicators of semantic and compositional complexity. Accordingly, we assign higher importance to these two factors by setting their weights (\emph{i.e.}, $w_1$ and $w_2$) to $0.2$, while assigning a weight of $0.1$ to the remaining seven semantic factors:

\vspace{-2mm}
\begin{equation}
w_j =
\begin{cases}
0.2, & j \in \{1,2\},\\
0.1, & j \in \{3,\ldots,9\}.
\end{cases}
\vspace{-0.8mm}
\end{equation}

We note that the absolute values of these weights are not critical, as the scores are used only to derive a relative ranking of prompts (based on $H(\cdot)$). Instead, the key design choice is the relative weighting scheme, which assigns approximately twice the importance to prompt length and object/attribute counts compared to the remaining factors. The resulting score serves as a heuristic estimate of prompt richness and compositional complexity. We compute this score for all \textit{candidate prompts}, rank them accordingly, and subsequently perform the prompt tiering procedure as described in \cref{supp:pt}.
