# Supplementary material for: DynEval: Holistic Evaluations of T2I Generative Models in the Wild
Source: arXiv:2607.11199 source file (2026-07-13)
Supplement: Supplementary file 5 [file 4_pt.tex]

\section{Prompt Tiering}
\label{supp:pt}

Given a set of $N$ candidate prompts $\{p_i\}_{i=1}^{N}$, we first compute a heuristic complexity score $h_i = H(p_i)$ for each prompt, where $H(\cdot)$ denotes the \textit{heuristic complexity scoring function} described in Sec.~\ref{supp:cbs}. We then sort the candidate prompts according to their complexity scores $\{h_i\}_{i=1}^{N}$ and partition the ranked distribution into three tiers corresponding to easy, medium, and hard prompts. This stratification enables \textbf{GenDB} to systematically capture a broad spectrum of semantic and compositional difficulties encountered in real-world text-to-image (T2I) generation. The score boundaries separating these tiers define two adaptive thresholds, $\tau_1$ and $\tau_2$, which are determined empirically from the score distribution rather than specified a priori. Importantly, the choice of $\tau_1$ and $\tau_2$ depends on several factors, including the \textit{size of the candidate prompt pool}, the \textit{desired number of complexity tiers}, and the \textit{capabilities of the target T2I models}. For instance, prompts with high semantic and compositional complexity can disproportionately challenge smaller open-source T2I models, often resulting in severe generation failures. Such prompt-image pairs are generally unsuitable for training the evaluator, as they provide limited opportunity to learn subtle semantic, compositional, and perceptual discrepancies.

Notably, during the construction of \textbf{GenDB}, we analyzed the complexity score distribution of the 1.8M prompts from DiffusionDB~\cite{DiffusionDB} and empirically selected $\tau_1 = 200$ and $\tau_2 = 100$, resulting in three prompt complexity tiers:
\vspace{-2mm}
\begin{equation}
\text{Tier}(p) =
\begin{cases}
\text{Tier-1 (Hard)} & \text{if } H(p) \ge \tau_1, \\
\text{Tier-2 (Medium)} & \text{if } \tau_2 \le H(p) < \tau_1, \\
\text{Tier-3 (Easy)} & \text{otherwise}
\end{cases}
\vspace{-2mm}
\end{equation}

In addition to the complexity-related metadata extraction described in Sec.~\ref{supp:cbs}, we employ \texttt{Qwen3-8B} to annotate each prompt with semantic dimension and subcategory labels based on a predefined taxonomy comprising 9 dimensions and 42 subcategories. Since a real-world prompt can simultaneously encompass multiple semantic concepts (\emph{e.g.}, objects, attributes, actions, spatial relationships, and artistic styles), we adopt a multi-label categorization strategy, assigning all applicable semantic dimensions and subcategory labels to each prompt. These semantic annotations are not used to determine the complexity tiers; rather, they are utilized during prompt selection within each tier. Specifically, after partitioning the 1.8M prompts into three complexity tiers, we perform diversity-aware sampling from each tier while ensuring broad coverage across all 42 semantic subcategories, yielding 500K prompts for \textbf{GenDB}. This strategy prevents the over-representation of frequent prompt types and enables GenDB to capture variations in both semantic content and compositional complexity.

\myparagraph{\textit{Illustrations of Prompt Tiering and Categorization.}}
Tab.~\ref{tab:tier_prompts} presents representative examples from each prompt complexity tier. As expected, Tier-1 primarily contains longer prompts with richer compositional structure and multiple semantic constraints, whereas Tier-3 consists of shorter prompts with relatively simple semantics. Tier-2 lies between these two extremes, containing prompts of moderate length and complexity. Representative examples covering the 42 prompt subcategories grouped under the 9 major semantic dimensions are presented in Tab.~\ref{tab:prompt_cat_1}--Tab.~\ref{tab:prompt_cat_5}. Specifically, Tab.~\ref{tab:prompt_cat_1} presents subcategories belonging to \textit{Object and Entity}; Tab.~\ref{tab:prompt_cat_2} covers \textit{Attribute Binding}; Tab.~\ref{tab:prompt_cat_3} includes \textit{Counting}, \textit{Spatial}, and \textit{Relations}; Tab.~\ref{tab:prompt_cat_4} illustrates \textit{Actions}, \textit{Scene Understanding}, and \textit{Text and Symbols}; and Tab.~\ref{tab:prompt_cat_5} presents subcategories from \textit{Style and Aesthetics}. For each subcategory, a representative prompt is provided, with the corresponding words or phrases highlighted for clarity.
\begin{table}[!t]
\centering
\caption{Illustrative prompts from the \grayhl{\textbf{\textit{Object and Entity}}} semantic dimension, one of the 9 dimensions in the considered prompt taxonomy. Representative prompts from the remaining semantic dimensions are presented in Tab.~\ref{tab:prompt_cat_2}--Tab.~\ref{tab:prompt_cat_5}. Words or phrases corresponding to each subcategory within this dimension are highlighted for clarity.}
\footnotesize
\begin{tabularx}{\textwidth}{p{3.6cm} p{3.6cm} >{\raggedright\arraybackslash}X}
\toprule
\textbf{Prompt Category} & \textbf{Subcategory} & \textbf{Prompt Example} \\
\midrule

Object and Entity & Single Object &
A \hlkw{single wooden chair} placed in the center of a white studio background \\

Object and Entity & Two Objects &
\hlkw{Two vipers entwined}, fighting to the death realistic cinematic 3 5 mm \\

Object and Entity & Human Present &
A portrait of \hlkw{a young woman} reading a book while sitting in a cozy café, warm lighting, coffee cup on the table, realistic photography, shallow depth of field, 8k \\

Object and Entity & Animal Present &
A \hlkw{golden retriever} running through a grassy park under a bright blue sky, joyful expression, motion blur, natural outdoor lighting, highly detailed, 8k photography \\

Object and Entity & Vehicle Present &
A \hlkw{blue sports car} parked beside a mountain road at sunset, cinematic lighting, dramatic clouds, photorealistic render, ultra detailed, 8k \\

Object and Entity & Food Present &
A \hlkw{bowl of ramen} with noodles, eggs, and vegetables on a wooden table, steam rising, food photography, studio lighting, hyper realistic, detailed textures \\

Object and Entity & Plant Present &
A \hlkw{green cactus} growing in a clay pot near a sunny window, minimal interior background, soft natural lighting, ultra detailed botanical photography \\

Object and Entity & Landmark Present &
\hlkw{The Eiffel Tower} illuminated at night with glowing city lights and reflections on the river Seine, cinematic view, long exposure photography, ultra detailed \\

\bottomrule
\end{tabularx}
\label{tab:prompt_cat_1}
\end{table}

\begin{table}[!t]
\centering
\caption{Illustrative prompts from the \grayhl{\textbf{\textit{Attribute Binding}}} semantic dimension, continuing Tab.~\ref{tab:prompt_cat_1}. Words or phrases corresponding to each subcategory within this dimension are highlighted for clarity.}
\footnotesize
\begin{tabularx}{\textwidth}{p{3.6cm} p{3.6cm} >{\raggedright\arraybackslash}X}
\toprule
\textbf{Prompt Category} & \textbf{Subcategory} & \textbf{Prompt Example} \\
\midrule

Attribute Binding & Atomic Color Binding &
A \hlkw{blue bicycle with bright red wheels} parked beside a white wall in a quiet street, vibrant colors, soft shadows, photorealistic, 8k \\

Attribute Binding & Shape Binding &
A \hlkw{triangular yellow kite} with blue stripes flying high in a clear sky above a grassy field, bright daylight, dynamic perspective \\

Attribute Binding & Material Binding &
A \hlkw{glass teapot with a polished metal handle} placed on a marble countertop with soft reflections, studio lighting, macro photography, ultra detailed \\

Attribute Binding & Texture Binding &
A \hlkw{fluffy white pillow} resting on a rough wooden bench inside a rustic cabin, soft sunlight through window, detailed texture contrast \\

Attribute Binding & Size Binding &
A \hlkw{tiny toy robot} standing next to a \hlkw{large cardboard box} on a clean floor, size contrast emphasis, studio lighting, photorealistic \\

Attribute Binding & Style Binding &
A portrait of a woman painted in \hlkw{impressionist style} with vibrant brushstrokes and colorful lighting, inspired by classic impressionist art \\

Attribute Binding & Multi Attribute Binding &
A \hlkw{small green frog wearing a red hat and holding a yellow umbrella} while sitting on a lily pad in a pond, whimsical fantasy illustration \\

\bottomrule
\end{tabularx}
\label{tab:prompt_cat_2}
\end{table}

\begin{table}[!t]
\centering
\caption{Illustrative prompts from the \grayhl{\textbf{\textit{Counting}}}, \grayhl{\textbf{\textit{Spatial}}}, and \grayhl{\textbf{\textit{Relations}}} semantic dimensions, continuing Tab.~\ref{tab:prompt_cat_2}. Words or phrases corresponding to each subcategory within these dimensions are highlighted for clarity.}
\footnotesize
\begin{tabularx}{\textwidth}{p{3.6cm} p{3.6cm} >{\raggedright\arraybackslash}X}
\toprule
\textbf{Prompt Category} & \textbf{Subcategory} & \textbf{Prompt Example} \\
\midrule

Counting & Count Exact &
\hlkw{Five bright oranges} arranged in a straight line on a kitchen table with soft window lighting, photorealistic food photography \\

Counting & Count Approx. &
\hlkw{About twenty birds} flying together across a glowing sunset sky above the ocean, dramatic clouds, cinematic atmosphere \\

Counting & Count Multi Objects &
\hlkw{Three dogs and two cats} sitting together in a cozy living room with a couch and warm lighting, cute and friendly scene \\

\midrule

Spatial & Spatial 2D &
A black cat sitting \hlkw{to the left of a red suitcase} on the floor inside an airport terminal, soft indoor lighting \\

Spatial & Spatial 3D &
A drone flying \hlkw{high above a forest valley} with mountains in the distance and mist in the air, aerial cinematic photography \\

Spatial & Relative Position &
A coffee cup placed \hlkw{behind a laptop} on a wooden desk with scattered notebooks and pens, cozy workspace lighting \\

Spatial & Perspective &
A busy city street viewed \hlkw{from a high rooftop looking down} at traffic and pedestrians, dramatic perspective, night lights \\

\midrule

Relations & Object Interaction &
A child \hlkw{throwing a ball to a dog} in a green park with trees and sunshine, action moment captured, natural lighting \\

Relations & Comparative Relation &
A \hlkw{tall giraffe standing next to a shorter zebra} in an African savanna landscape during golden hour \\

Relations & Multi Relation &
A \hlkw{man handing a book to a woman while a child watches} in a library filled with bookshelves and warm lighting \\

\bottomrule
\end{tabularx}
\label{tab:prompt_cat_3}
\end{table}

\begin{table}[!t]
\centering
\caption{Illustrative prompts from the \grayhl{\textbf{\textit{Actions}}}, \grayhl{\textit{\textbf{Scene Understanding}}}, and \grayhl{\textit{\textbf{Text and Symbols}}} semantic dimensions, continuing Tab.~\ref{tab:prompt_cat_3}. Words or phrases corresponding to each subcategory within these dimensions are highlighted for clarity.}
\footnotesize
\begin{tabularx}{\textwidth}{p{3.6cm} p{3.6cm} >{\raggedright\arraybackslash}X}
\toprule
\textbf{Prompt Category} & \textbf{Subcategory} & \textbf{Prompt Example} \\
\midrule

Actions & Human Action &
A chef \hlkw{chopping vegetables} on a kitchen counter with knives and ingredients spread around, culinary action photography \\

Actions & Animal Action &
A cat \hlkw{jumping from a chair onto a wooden table} inside a bright kitchen, motion captured mid-air \\

Actions & Object Manipulation &
A robotic arm \hlkw{assembling a smartphone} on a futuristic factory assembly line, glowing lights, advanced technology scene \\

\midrule

Scene Understanding & Indoor Scene &
A \hlkw{cozy living room interior} with sofa, lamp, bookshelf, and soft warm lighting, realistic interior photography \\

Scene Understanding & Outdoor Scene &
People walking through a \hlkw{busy outdoor street market} with colorful stalls, fruits, fabrics, and vibrant atmosphere \\

Scene Understanding & Urban Scene &
A \hlkw{dense urban city skyline} filled with skyscrapers and busy traffic during sunset, cinematic lighting, ultra detailed \\

Scene Understanding & Natural Scene &
A \hlkw{calm lake surrounded by pine trees and mountains} reflecting in the water during sunrise, peaceful natural landscape \\

\midrule

Text and Symbols & Text in Image &
A street sign clearly displaying the word \hlkw{STOP} in bright red letters at a city intersection \\

Text and Symbols & Symbol Rendering &
A glowing neon \hlkw{peace symbol} mounted on a dark brick wall in a nighttime urban alley \\

Text and Symbols & Logo or Sign &
High quality simplified rectangular \hlkw{logo of a medieval stone blacksmith forge} shaped like a realistic dragon head looking at viewer, for a company called poly - forge, symmetrical!!!, award winning, art deco!!!!!! by milton glaser \\

\bottomrule
\end{tabularx}
\label{tab:prompt_cat_4}
\end{table}

\begin{table}[!t]
\centering
\caption{Illustrative prompts from the \grayhl{\textbf{\textit{Style and Aesthetics}}} semantic dimension, continuing Tab.~\ref{tab:prompt_cat_4}. Words or phrases corresponding to each subcategory within this dimension are highlighted for clarity.
}
\footnotesize
\begin{tabularx}{\textwidth}{p{3.6cm} p{3.6cm} >{\raggedright\arraybackslash}X}
\toprule
\textbf{Prompt Category} & \textbf{Subcategory} & \textbf{Prompt Example} \\
\midrule

Style and Aesthetics & Art Style &
A heroic warrior portrait illustrated in \hlkw{medieval fantasy art style}, detailed armor, dramatic lighting, epic composition \\

Style and Aesthetics & Photographic Style &
A professional \hlkw{portrait photograph} of a woman with soft lighting and shallow depth of field, studio photography \\

Style and Aesthetics & Artist Style &
A portrait painting of a woman in the style of \hlkw{Vincent van Gogh} with expressive brush strokes and vivid colors \\

Style and Aesthetics & Genre Style &
A retro \hlkw{science fiction poster} showing a spaceship flying over a futuristic city in bold 1980s illustration style \\

Style and Aesthetics & Surreal Scene &
A \hlkw{surreal floating island} in the sky with upside down waterfalls and glowing crystals, fantasy concept art \\

Style and Aesthetics & Anti-realism &
A \hlkw{rhombohedral, cubist} small pink square with an irregular diagonal, and white triangle above it by jacques villon, trending on flickr, crystal cubism, angular, cubism, geometric. \\

Style and Aesthetics & Fantasy Content &
A \hlkw{dragon flying over a castle} during a stormy night, lightning in the sky, epic fantasy digital painting \\

\bottomrule
\end{tabularx}
\label{tab:prompt_cat_5}
\end{table}
