# Supplementary material for: DynEval: Holistic Evaluations of T2I Generative Models in the Wild
Source: arXiv:2607.11199 source file (2026-07-13)
Supplement: Supplementary file 6 [file 5_mt.tex]

\section{Model Tiering}
\label{supp:mt}

Tab.~\ref{tab:dyneval_models} reports the complete ranking of the \textbf{36} T2I models considered in DynEval, along with their DynEval scores and corresponding tier assignments. Following \cref{sec:gendb} of the main paper, each T2I model is evaluated on the DynEval-1K evaluation set by averaging the teacher model's predicted DynEval scores over 1,000 generated prompt-image pairs. Based on these scores, the models are partitioned into three capability tiers using two empirically selected thresholds ($\mu_1$ and $\mu_2$), where Tier-1 denotes the strongest models and Tier-3 the weakest. The proposed tiering serves two complementary purposes. First, it enables the \textit{tier-matched prompt-model generation} strategy adopted during GenDB construction, where Tier-1, Tier-2, and Tier-3 models are paired with hard, medium, and easy prompts, respectively. Since weaker models often struggle even with simpler prompts whereas stronger models rarely fail on easier prompts, matching model capability with prompt complexity results in a broader and more diverse set of semantic and perceptual failure cases. Second, the tier assignments facilitate the fine-grained analysis of model capabilities presented in \cref{fig:category_score} of the main paper by additionally comparing the best-performing (Fig.~\ref{fig:category_score_best}) and worst-performing (Fig.~\ref{fig:category_score_worst}) models from each tier across the 42 prompt subcategories.

On the DynEval-1K evaluation set, Tier-1, Tier-2, and Tier-3 models achieve average DynEval scores of $0.872 \pm 0.041$, $0.739 \pm 0.039$, and $0.528 \pm 0.123$, respectively. The tier thresholds are selected empirically by analyzing the score distribution in Tab.~\ref{tab:dyneval_models}; specifically, we define two thresholds, $\mu_1$ and $\mu_2$ ($\mu_1 > \mu_2$), and set them to \textbf{0.81} and \textbf{0.67}, respectively. Notably, these thresholds should be interpreted as relative groupings rather than universal performance boundaries, since different prompt distributions or T2I model pools would naturally produce different score distributions and, consequently, different threshold values.
\begin{table}[!t]
\centering

\caption{
\textbf{Overall performance of 36 T2I models on the DynEval-1K evaluation set.} Models are ordered according to the teacher model's predicted DynEval score (normalized to $[0,1]$) and grouped into three capability tiers. We also report the mean and standard deviation of each tier.
}

\footnotesize
\vspace{-2mm}
\setlength{\tabcolsep}{7pt}
\begin{tabular}{l | c | c |c}
\toprule
\textbf{Model} & \textbf{Tier} & \textbf{DynEval Score} & \textbf{Avg $\pm$ Std} \\
\midrule

GPT-Image-1.5~\cite{gpt_image_1_5} & \multirow{7}{*}{TIER-1} & 0.934 & \multirow{7}{*}{0.872 $\pm$ 0.041} \\
NanoBanana~\cite{team2023gemini} & & 0.915 & \\
FLUX.2 [klein]~\cite{flux-2-2025} & & 0.883 & \\
FLUX.2 [dev]~\cite{flux-2-2025} & & 0.866 & \\
FIBO~\cite{gutflaish2025generating} & & 0.844 & \\
LongCat-Image~\cite{LongCat-Image} & & 0.834 & \\
HiDream-I1~\cite{hidreami1technicalreport} & & 0.830 & \\

\midrule

Qwen-Image~\cite{wu2025qwen} & \multirow{19}{*}{TIER-2} & 0.793 & \multirow{19}{*}{0.739 $\pm$ 0.039} \\
Z-Image~\cite{team2025zimage} & & 0.789 & \\
GLM-Image~\cite{glmimage2024} & & 0.780 & \\
FLUX.1 [dev]~\cite{labs2025flux1kontextflowmatching} & & 0.776 & \\
Sana~\cite{xie2024sana} & & 0.769 & \\
UniPic~\cite{wang2025skywork} & & 0.768 & \\
Stable Diffusion 3.5~\cite{esser2024scaling} & & 0.767 & \\
OmniGen2~\cite{wu2025omnigen2} & & 0.765 & \\
In-Context LoRA~\cite{huang2024context} & & 0.757 & \\
Bagel~\cite{deng2025bagel} & & 0.755 & \\
OmniGen~\cite{xiao2025omnigen} & & 0.741 & \\
Hunyuan-DiT~\cite{li2024hunyuan_dit} & & 0.727 & \\
Show-o~\cite{xie2024show} & & 0.711 & \\
X-Omni~\cite{geng2025x} & & 0.706 & \\
Janus-Pro~\cite{chen2025janus} & & 0.696 & \\
Kolors~\cite{kolors} & & 0.689 & \\
PixArt-$\alpha$~\cite{chen2023pixart} & & 0.685 & \\
Kandinsky 3~\cite{arkhipkin2023kandinsky} & & 0.683 & \\
UniWorld-V1~\cite{lin2025uniworld} & & 0.682 & \\

\midrule

Playground v2.5~\cite{li2024playground} & \multirow{10}{*}{TIER-3} & 0.655 & \multirow{10}{*}{0.528 $\pm$ 0.123} \\
SSD-1B~\cite{gupta2024progressive} & & 0.613 & \\
DeepFloyd IF-XL~\cite{deepfloydif2023} & & 0.609 & \\
Emu3~\cite{wang2024emu3} & & 0.597 & \\
SDXL-Turbo~\cite{podell2023sdxl} & & 0.594 & \\
Stable Diffusion XL~\cite{podell2023sdxl} & & 0.553 & \\
Stable Diffusion v2.1~\cite{rombach2022high} & & 0.523 & \\
Stable Diffusion v1.5~\cite{rombach2022high} & & 0.475 & \\
PixArt-$\Sigma$~\cite{chenweak} & & 0.425 & \\
LlamaGen~\cite{sun2024autoregressive} & & 0.240 & \\

\bottomrule
\end{tabular}

\label{tab:dyneval_models}
\vspace{-5mm}
\end{table}
