# Supplementary material for: DynEval: Holistic Evaluations of T2I Generative Models in the Wild
Source: arXiv:2607.11199 source file (2026-07-13)
Supplement: Supplementary file 7 [file 6_tier_threshold.tex]

\section{Details on Tier-Specific Thresholds}
\label{supp:tst}

As described in \cref{sec:gendb} of the main paper, GenDB is constructed using the proposed \textit{tier-matched prompt-model pairing} strategy. Building upon GenDB, \cref{sec:DynEvalInstruct} introduces a second-stage curation process to construct DynEvalInstruct using teacher-generated T2IA and IQA responses. For each prompt-image pair, the T2IA and IQA scores are obtained from the teacher model's responses and combined into a single scalar score: $S = 0.5 \times S_{\mathrm{T2IA}} + 0.5 \times S_{\mathrm{IQA}}$. Since GenDB contains images generated by three T2I model tiers with different performance ranges, the curation framework employs tier-specific selection thresholds $\delta_i$, where $i \in \{1,2,3\}$. A sample generated by a Tier-$i$ model is retained if $S < \delta_i$. In practice, we found that a common threshold was sufficient across all tiers and therefore set $\delta_1 = \delta_2 = \delta_3 = 5$. Since the maximum possible combined score is $S=5$, this criterion removes only prompt-image pairs that receive the highest possible score. Such samples typically exhibit near-perfect text-image alignment and visual quality, providing limited supervision for learning fine-grained evaluator behavior. Consequently, we retain only samples satisfying $S<5$, which are more likely to contain semantic, compositional, or perceptual discrepancies that serve as informative training examples. Applying this filtering strategy to GenDB yields the final 250K-sample DynEvalInstruct dataset. Notably, as shown in Sec.~\ref{supp:data_scaling}, evaluator performance begins to saturate at approximately 250K training samples, with only marginal improvements beyond this point.
