# Supplementary material for: DynEval: Holistic Evaluations of T2I Generative Models in the Wild
Source: arXiv:2607.11199 source file (2026-07-13)
Supplement: Supplementary file 8 [file 7_ablation.tex]

\section{Additional Ablation Study}
\label{supp:aas}

\begin{wraptable}[15]{r}{0.6\textwidth}
\vspace{-12mm}
\centering
\caption{\textbf{Ablation on teacher model selection.} Average DynEval score (mean $\pm$ standard deviation) for different teacher model candidates evaluated on the DynEval-1K evaluation set. Scores are normalized to the range $[0,1]$. Lower scores correspond to stricter evaluators and are therefore preferred for knowledge distillation.}
\label{tab:teacher_ablation}

\small
\resizebox{0.6\columnwidth}{!}{%
\begin{tabular}{lc}
\toprule
\textbf{Model} & \textbf{DynEval Score} ($\downarrow$) \\
\midrule

Qwen3-VL-235B-A22B-Instruct~\cite{Bai2025qwen} & $0.850 \pm 0.192$ \\
GPT-5.1~\cite{gpt51_openai_2025} & $0.863 \pm 0.216$ \\
InternVL3.5-241B-A28B~\cite{wang2025internvl3}  & $0.900 \pm 0.100$ \\
InternVL3-78B~\cite{zhu2025internvl3} & $0.920 \pm 0.084$ \\
Qwen3-VL-32B-Instruct~\cite{Bai2025qwen} & $0.929 \pm 0.076$ \\
Qwen3-VL-8B-Instruct~\cite{Bai2025qwen} & $0.971 \pm 0.076$ \\
\bottomrule
\end{tabular}}
\vspace{-8pt}
\end{wraptable}
\subsection{Teacher Model Selection}
\label{supp:teacher_choice}
While \cref{tab:main_comp} in the main paper presents the student model ablation, here we provide additional ablations on the teacher model selection and investigate the effect of data scaling during fine-tuning. In Tab.~\ref{tab:teacher_ablation}, we report the average scores of different teacher model candidates evaluated on the DynEval-1K evaluation set. As a text-to-image evaluator, the teacher model should ideally adopt a stricter perspective, penalizing generated images when necessary and assigning lower scores accordingly. From Tab.~\ref{tab:teacher_ablation}, we observe that \texttt{Qwen3-VL-235B}~\cite{Bai2025qwen} best satisfies this criterion and is therefore the most suitable teacher model for distillation.

\subsection{Training Data Scaling}
\label{supp:data_scaling}

\begin{wraptable}[18]{r}{0.36\textwidth}
\vspace{-12mm}
\centering
\caption{\textbf{Ablation on training data scaling.} Performance of the DynEval-4B evaluator trained with different amounts of DynEvalInstruct data, evaluated using SRCC (mean $\pm$ standard deviation) on the TIFA~\cite{tifa} dataset. Scores are normalized to the range $[0,1]$. Correlation with human judgments improves consistently with increasing training set size and begins to saturate at approximately 250K training samples.}
\label{tab:data_scaling}

\small
\resizebox{0.35\columnwidth}{!}{%
\begin{tabular}{cc}
\toprule
\textbf{Training Data} & \textbf{SRCC} ($\uparrow$) \\
\midrule
50K  & $0.687 \pm 0.023$ \\
100K & $0.700 \pm 0.018$ \\
150K & $0.750 \pm 0.007$ \\
200K & $0.790 \pm 0.010$ \\
250K & $0.800 \pm 0.003$ \\
\bottomrule
\end{tabular}}
\vspace{-8pt}
\end{wraptable}
Tab.~\ref{tab:data_scaling} presents the training data scaling ablation for our DynEval-4B evaluator. As the size of the DynEvalInstruct training data increases from 50K to 250K samples, the Spearman Rank Correlation Coefficient (SRCC) with human judgments improves consistently, demonstrating the effectiveness of scaling supervision without relying on human-annotated data. Notably, performance begins to saturate at approximately 250K training samples, indicating diminishing returns beyond this point.
