# Supplementary material for: DynEval: Holistic Evaluations of T2I Generative Models in the Wild
Source: arXiv:2607.11199 source file (2026-07-13)
Supplement: Supplementary file 9 [file 8_more_results.tex]

\section{Additional Qualitative Results}
\label{supp:added_visual_results}

\begin{figure}[!t]
    \centering
    \includegraphics[width=\linewidth]{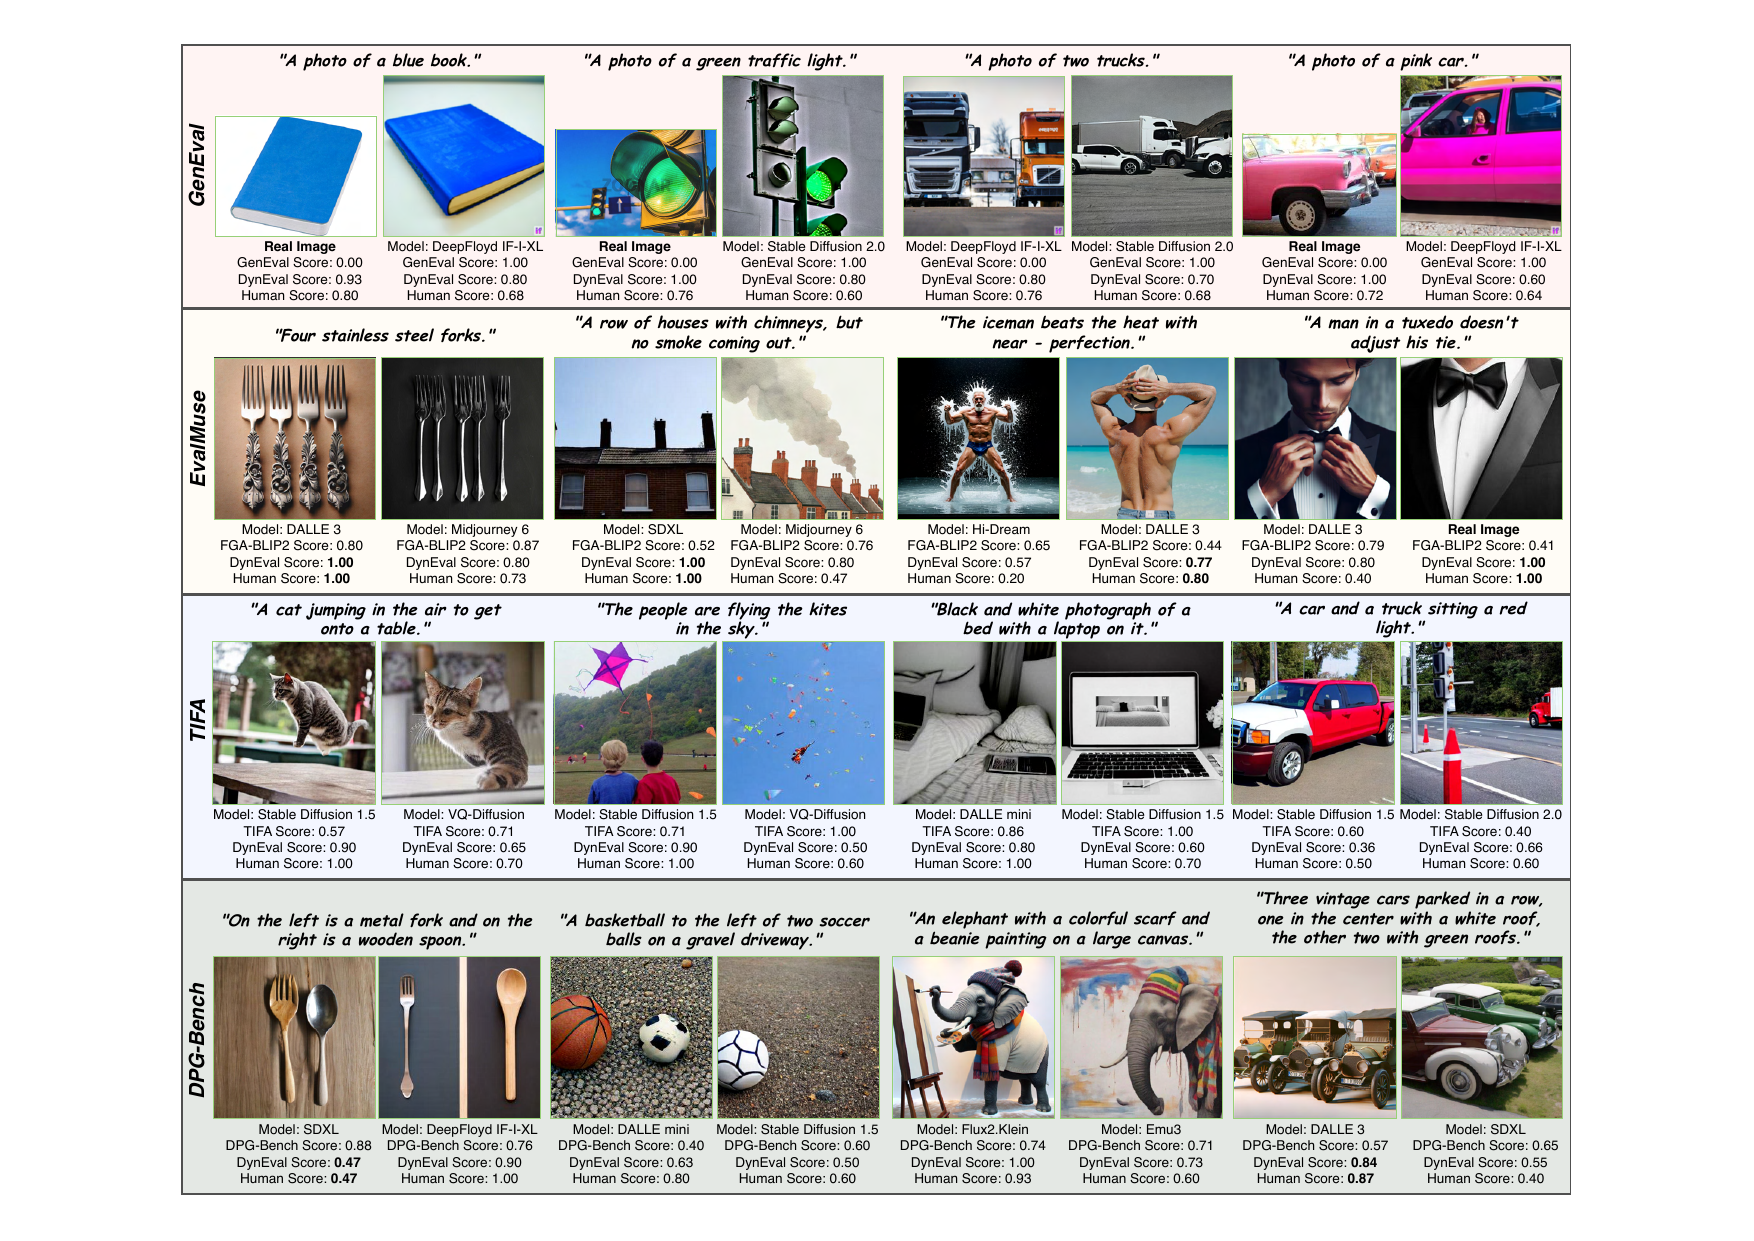}
    \vspace{-6mm}
    \caption{
    \textbf{Additional qualitative comparisons extending \cref{fig:qualitative_comp} in the main paper.} Comparison of DynEval-4B with representative T2I evaluation methods, including GenEval~\cite{GenEval}, TIFA~\cite{tifa}, DPG-Bench~\cite{DPGBench}, and EvalMuse~\cite{EvalMuse-40k}, together with human ratings. All scores are normalized to the range $[0,1]$ for fair comparison. The examples highlight representative failure cases of existing T2I evaluators, including detector dependency (GenEval~\cite{GenEval}), inaccurate semantic scoring (TIFA~\cite{tifa} and DPG-Bench~\cite{DPGBench}), and difficulties with negation and counting (EvalMuse~\cite{EvalMuse-40k}), while demonstrating that DynEval consistently produces scores that more closely align with human judgments by jointly evaluating text-image alignment and image quality.}
    \label{fig:supp_teaser_fig}
    \vspace{-5mm}
    
\end{figure}

In Fig.~\ref{fig:supp_teaser_fig}, we present additional qualitative comparisons that extend \cref{fig:qualitative_comp} from the main paper between DynEval and four representative T2I evaluation methods: GenEval~\cite{GenEval}, TIFA~\cite{tifa}, DPG-Bench~\cite{DPGBench}, and EvalMuse~\cite{EvalMuse-40k}. For a fair visual comparison, the scores from all evaluators, together with the human ratings, are normalized to the range $[0,1]$. GenEval~\cite{GenEval} evaluates object-centric compositional properties such as object presence, object count, color, and spatial relationships by leveraging an object detection model together with CLIP~\cite{radford2021learning}. However, because it relies heavily on the performance of the underlying object detector, it often fails to detect the presence of an object even when it is clearly visible in both the real and generated images, as illustrated in Fig.~\ref{fig:supp_teaser_fig}. This detector-dependent design limits GenEval's evaluation capability. TIFA~\cite{tifa} extends this paradigm through prompt-derived VQA-based T2I assessment, while DPG-Bench~\cite{DPGBench} emphasizes dense prompts involving multiple objects, attributes, and relationships by leveraging DSG~\cite{cho2023davidsonian}. However, these two approaches focus only on evaluating semantic alignment and do not explicitly account for perceptual image quality, resulting in two major contradictions: (i) visually superior images may receive disproportionately low scores, and (ii) visually distorted or semantically implausible images may receive overly high scores, as shown in Fig.~\ref{fig:supp_teaser_fig}. EvalMuse~\cite{EvalMuse-40k} further improves alignment evaluation through fine-grained prompt decomposition and the training of a T2I evaluator using 40K human-annotated ratings. However, the resulting evaluator often struggles with negation prompts and counting tasks involving multiple objects, as depicted in Fig.~\ref{fig:supp_teaser_fig}, highlighting the need for large-scale prompt exposure during evaluator training. In contrast, DynEval jointly evaluates text-image alignment (T2IA) and image quality assessment (IQA), enabling it to distinguish images with similar semantic correctness but substantially different visual quality. Trained on 250K samples without relying on human annotations, DynEval produces scores that more closely follow human judgments across the diverse examples shown in Fig.~\ref{fig:supp_teaser_fig}, often matching the human score exactly.
