# Supplementary material for: DynEval: Holistic Evaluations of T2I Generative Models in the Wild
Source: arXiv:2607.11199 source file (2026-07-13)
Supplement: Supplementary file 10 [file 9_failure.tex]

\section{Understanding Failure Attributes of T2I Models}
\label{supp:failure}

\cref{fig:category_score} of the main paper reports the average DynEval-4B predicted scores for Tier-1, Tier-2, and Tier-3 models across all 42 prompt subcategories in the DynEval-1K evaluation set. While these averages provide a high-level comparison across the three tiers, they do not capture the variability among models within the same tier. To better understand this intra-tier variation, Fig.~\ref{fig:category_score_best} and Fig.~\ref{fig:category_score_worst} present the highest-scoring and lowest-scoring models from each tier across all prompt subcategories. Specifically, \texttt{GPT-Image-1.5}, \texttt{Qwen-Image}~\cite{wu2025qwen}, and \texttt{Playground v2.5}~\cite{li2024playground} emerge as the best-performing models in Tier-1, Tier-2, and Tier-3, respectively, as shown in Fig.~\ref{fig:category_score_best}. Although these models exhibit consistently strong performance across most semantic dimensions, they show noticeable performance degradation on certain subcategories. Moreover, Fig.~\ref{fig:category_score_worst} highlights the weakest-performing model within each tier, revealing substantially lower performance across nearly all semantic dimensions. For example, \texttt{LlamaGen}~\cite{sun2024autoregressive}, the weakest Tier-3 model, consistently struggles with both object-centric prompts and more challenging compositional reasoning tasks. Nevertheless, the considerable performance gap between the best-performing and worst-performing models does not alter the relative ordering of the most challenging prompt categories, which remains remarkably consistent across all tiers. Notably, subcategories such as \textit{human present}, \textit{count multi objects}, \textit{size binding}, \textit{perspective}, \textit{anti-realism}, and \textit{text in image} remain among the lowest-scoring subcategories regardless of overall model strength, indicating that these semantic capabilities continue to be challenging for current T2I models.

Overall, these results demonstrate that the proposed tier assignments effectively capture broad differences in model capability while preserving meaningful variation among models within the same tier. They also show that models with comparable overall DynEval scores can still exhibit distinct strengths and weaknesses across individual semantic dimensions, motivating fine-grained category-wise analysis in addition to overall benchmark performance.

\begin{figure}[!t]
    \centering
    \includegraphics[width=\linewidth]{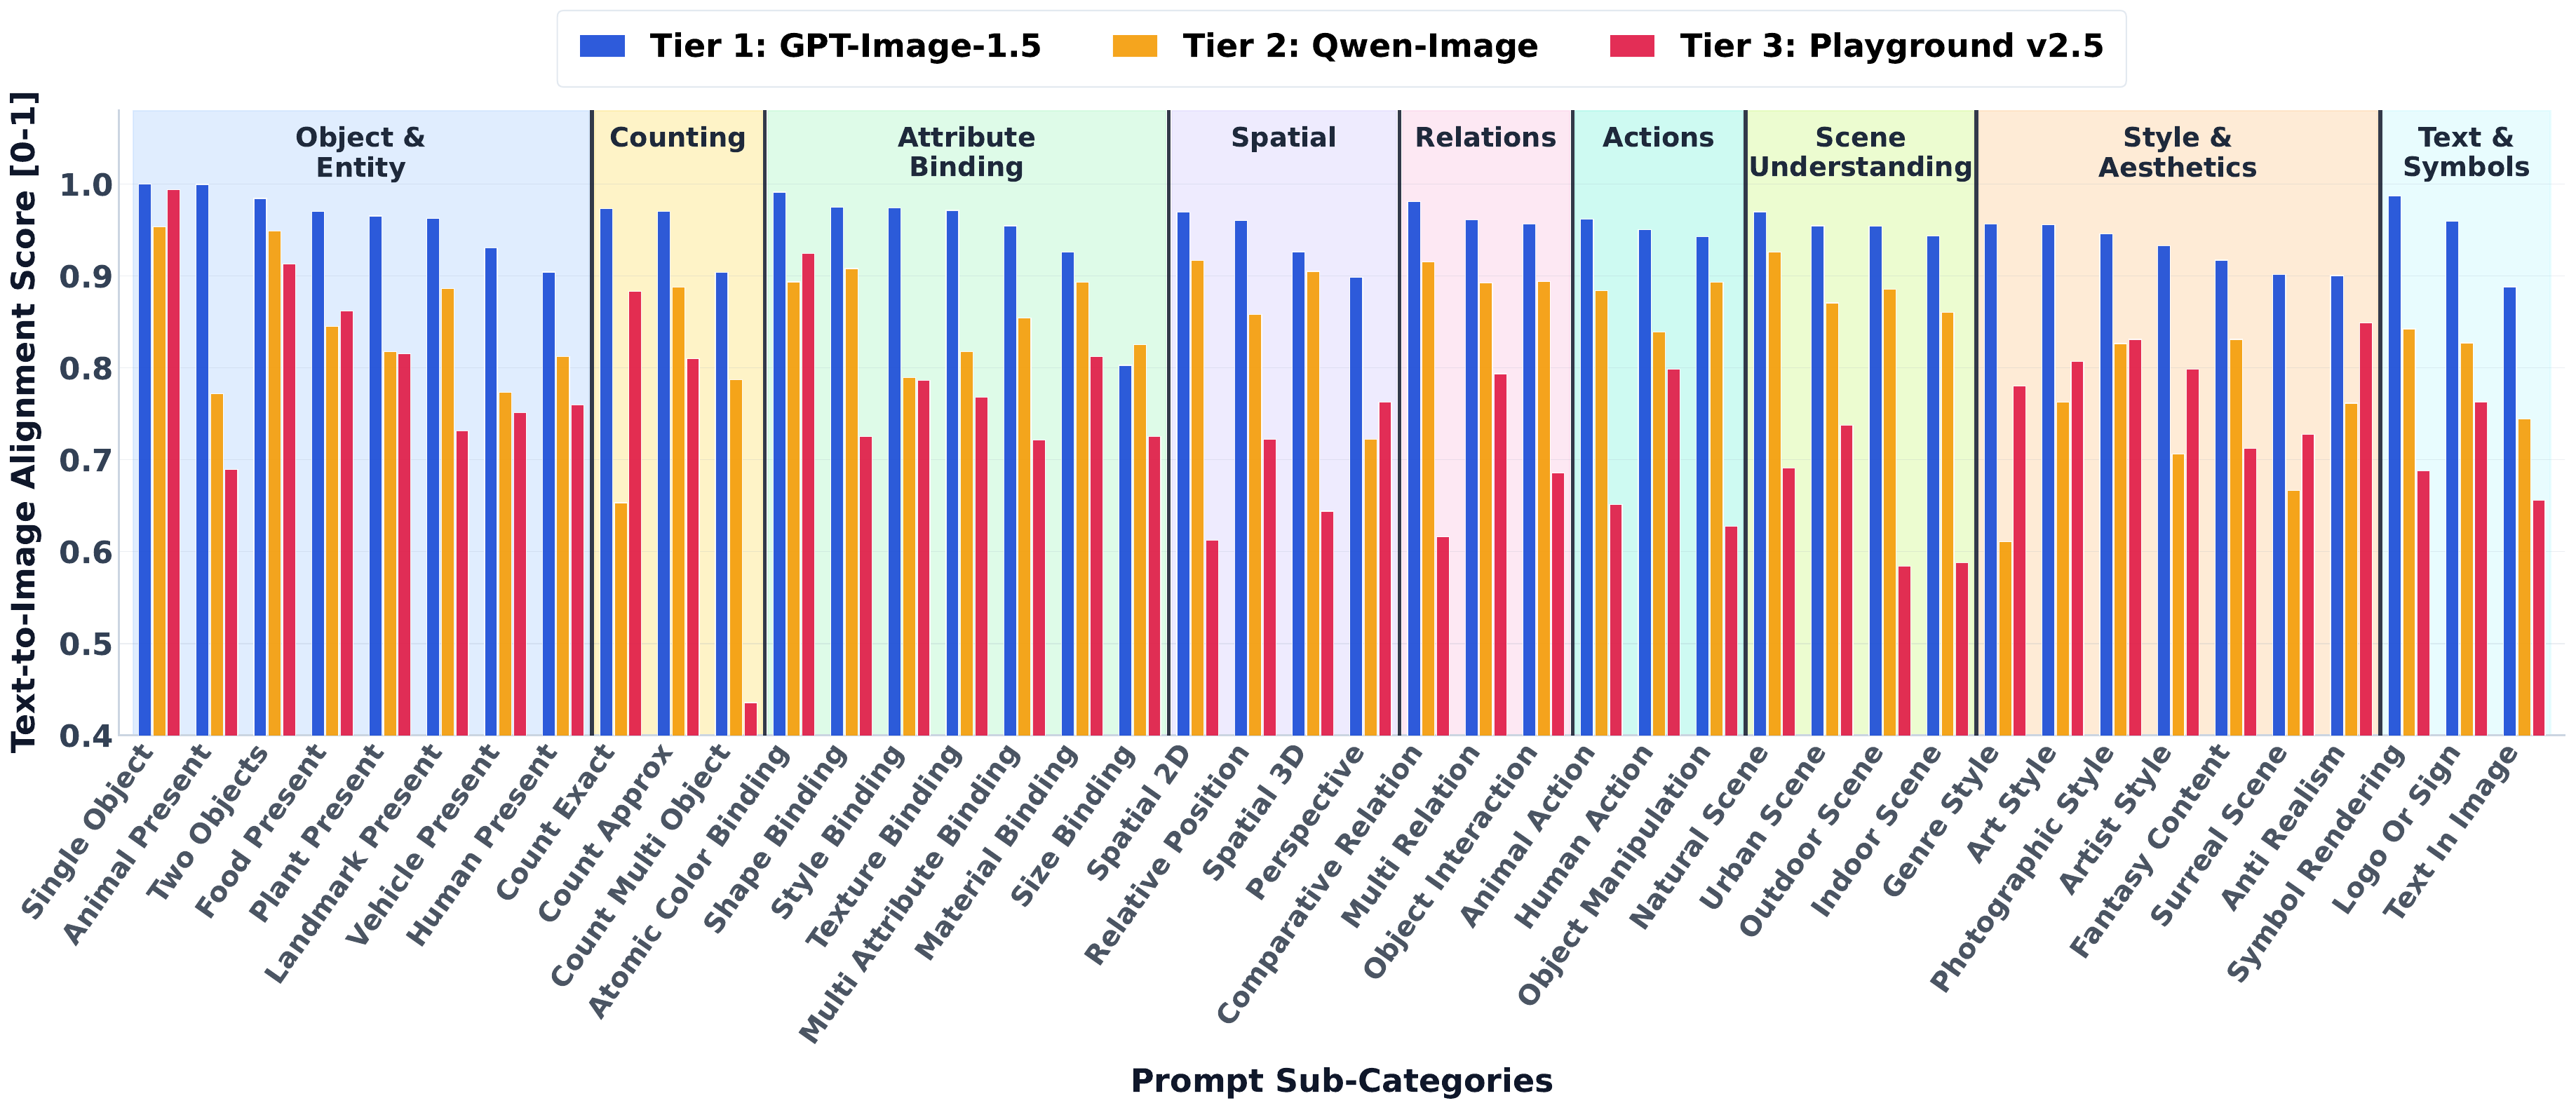} 
    \caption{Performance of the \textbf{best-scoring model} from each model tier across the 42 prompt subcategories on the \textbf{DynEval-1K} evaluation set. GPT-Image-1.5~\cite{gpt_image_1_5}, Qwen-Image~\cite{wu2025qwen}, and Playground v2.5~\cite{li2024playground} are the highest-ranked models in Tier-1, Tier-2, and Tier-3, respectively, based on their DynEval-4B predicted scores. Although these models achieve consistently strong performance across most semantic dimensions, they continue to exhibit noticeable weaknesses on challenging subcategories such as \textit{human present}, \textit{count multi objects}, \textit{size binding}, \textit{perspective}, \textit{anti-realism}, and \textit{text in image}.}
    \label{fig:category_score_best}
\end{figure}

\begin{figure}[!t]
    \centering
    \includegraphics[width=\linewidth]{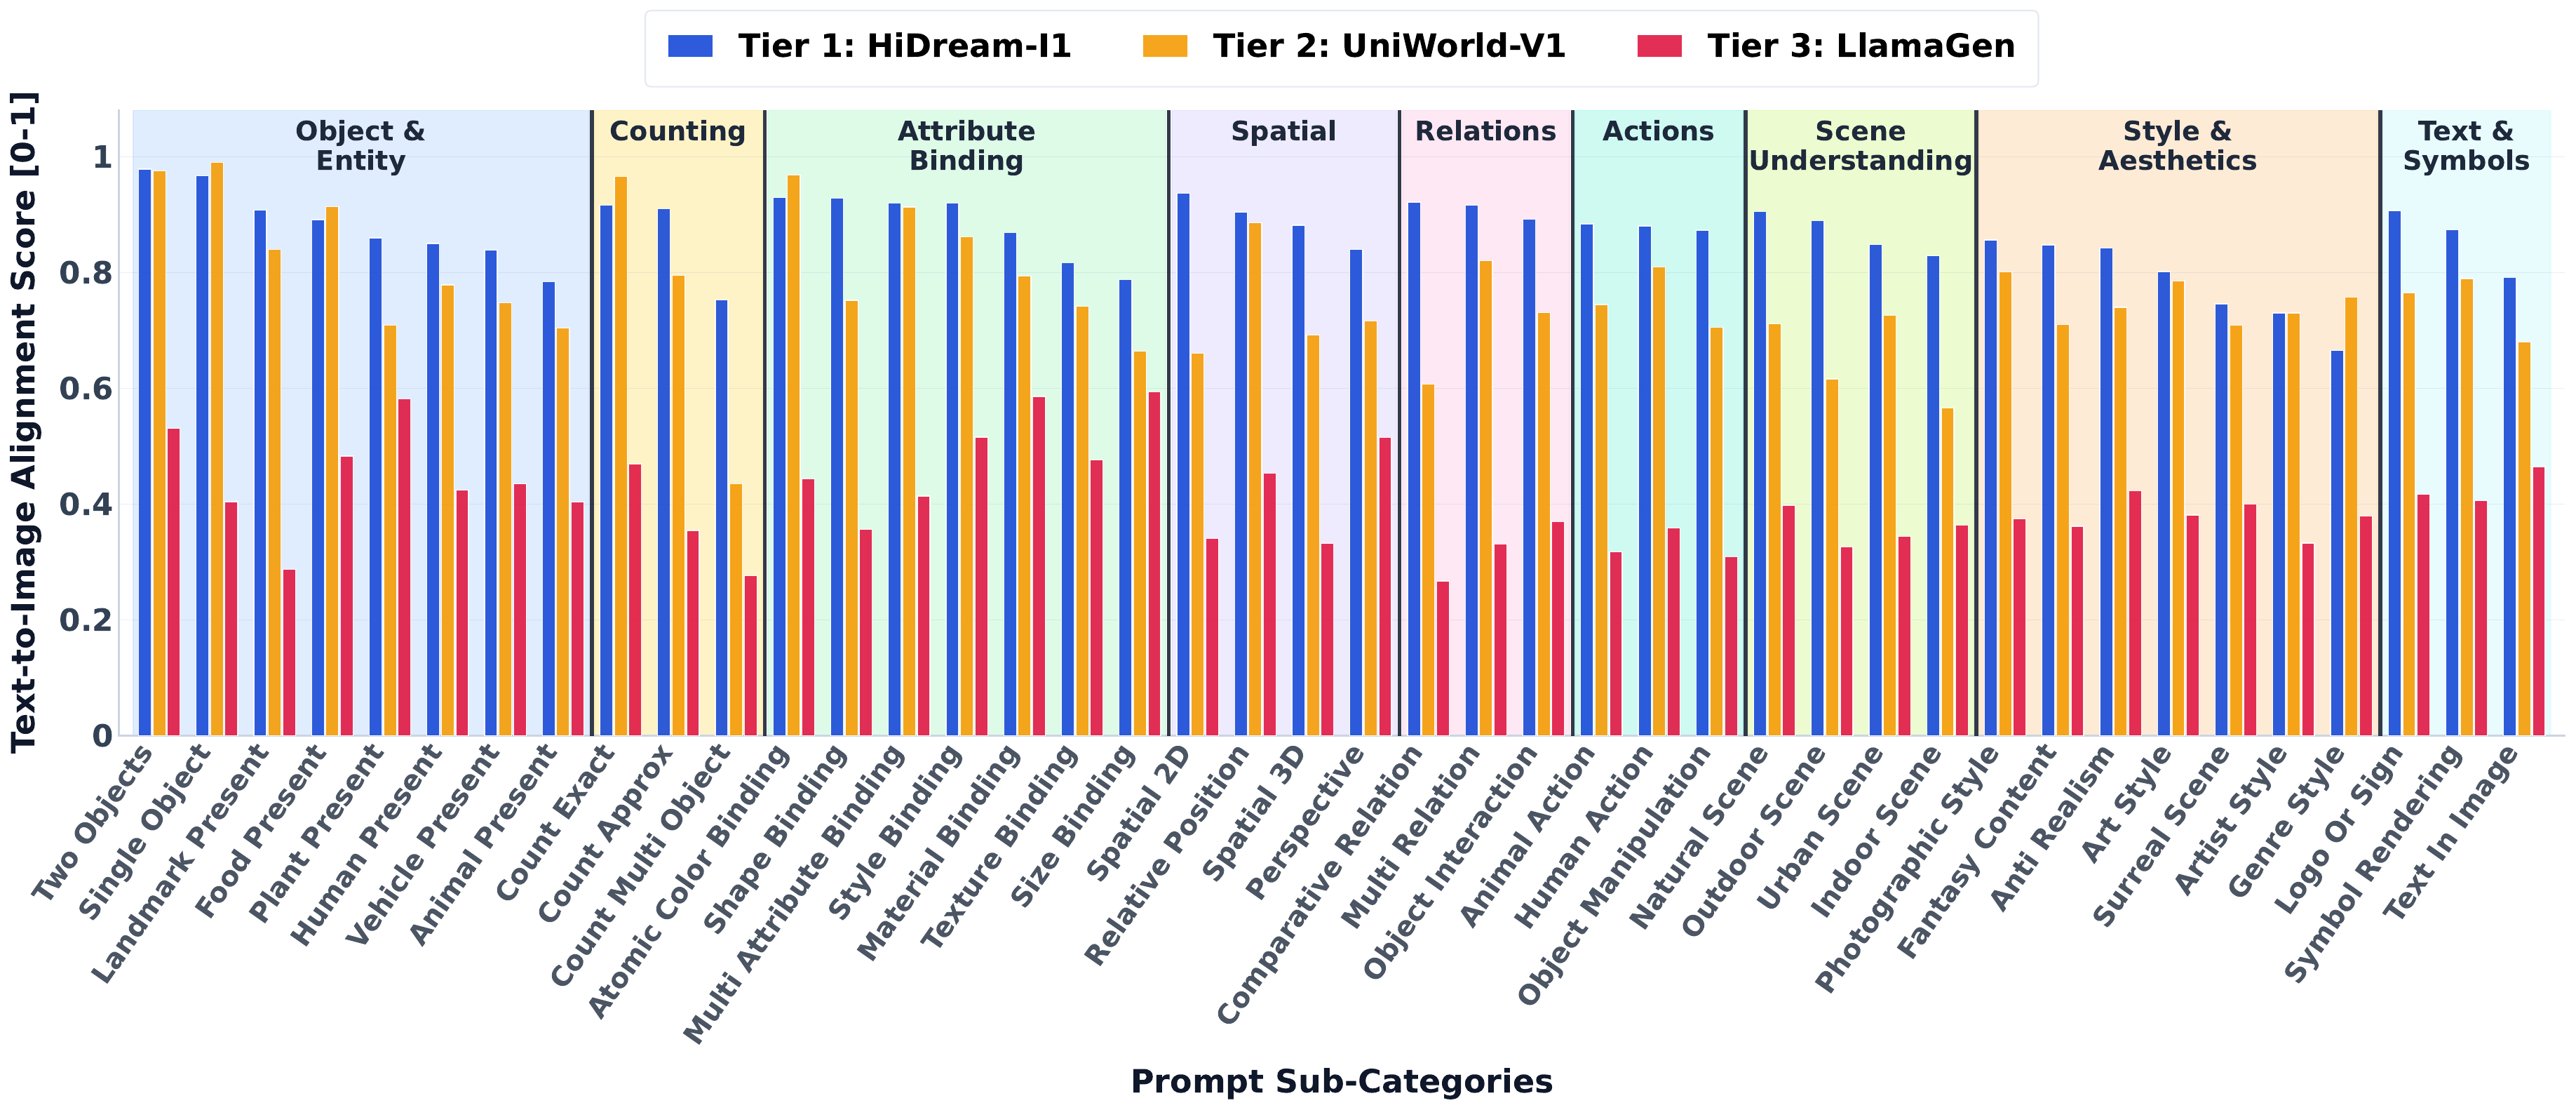}
    \caption{Performance of the \textbf{lowest-scoring model} from each model tier across the 42 prompt subcategories on the \textbf{DynEval-1K} evaluation set. HiDream-I1~\cite{hidreami1technicalreport}, UniWorld-V1~\cite{lin2025uniworld}, and LlamaGen~\cite{sun2024autoregressive} are the lowest-ranked models in Tier-1, Tier-2, and Tier-3, respectively, based on their DynEval-4B predicted scores. These models exhibit substantially lower performance across nearly all semantic dimensions, while the relative ordering of the most challenging prompt subcategories remains largely consistent across all model tiers.}
    \label{fig:category_score_worst}
    \vspace{-5mm}
\end{figure}
